# Supplementary material for: Characterizing the Role of Peierls Vibrations in Singlet Fission with the Adaptive Hierarchy of Pure States
Source: arXiv:2505.02292 ancillary file (2025-06-23)
Supplement: Supplementary file 1 [file SI.pdf]

# Characterizing the Role of Peierls Vibrations in Singlet Fission with the Adaptive Hierarchy of Pure States: Supporting Information

Jacob K. Lynd[1] and Doran I.G.B. Raccah[1]
*Department of Chemistry, University of Texas at Austin, Austin, TX, 78712, USA*

(Dated: 23 June 2025)

## CONTENTS

**S1. The adHOPS Algorithm** S2
A. The adHOPS Wave Function S2
B. The HOPS Equation-of-Motion S2
C. Redefinition of Terms S4
D. The Adaptive Algorithm S5

**S2. Error Calculations** S6
A. Adaptive Auxiliary Basis S7
1. Stable Auxiliary Basis S8
2. Boundary Auxiliary Basis S9
B. Adaptive State Basis S10
1. Stable State Basis S11
2. Boundary State Basis S12

**S3. Drude-Lorentz Spectral Density** S13

**S4. Size-Invariance in Various Models** S14

**S5. The PDI Hamiltonian** S15
A. MSD Calculations S17

**S6. Effective Couplings in the PDI Model** S18
A. J-Aggregate-Like Singlet Nearest-Neighbor Coupling S18
B. Effective Coupling of the CT-Mediated Mechanism S19

**S7. Convergence** S19
A. Calculation Parameters S19
1. Hierarchy Depth $k_{\mathrm{max}}$ S19
2. Number of Matsubara Modes $k_{\mathrm{Mats}}$ S19
3. Integration Time Step $dt$ S20
4. Adaptive Error Bounds $\delta_A$ and $\delta_S$ S20
5. Basis Update Time $u_t$ S20
6. Ensemble Size $N_{\mathrm{traj}}$ S20
7. Discard Fraction ($f_{\mathrm{dis}}$) S20
8. Early Time Basis Construction S20
9. Effective Integration of the Noise S20
B. Convergence Testing S20
1. Peierls Linear Chain Model S21
2. Singlet Fission in PDI S21

# S1. THE ADHOPS ALGORITHM

## A. The adHOPS Wave Function

The adaptive Hierarchy of Pure States (adHOPS)[1] is a reduced-scaling implementation of HOPS,[2] a method for solving a stochastic unravelling of the dynamics of an open quantum system described by the Hamiltonian

$$\hat{H} = \hat{H}_{\mathrm{S}} + \sum_{n,q_n} \Lambda_{q_n} \hat{L}_n (\hat{a}^\dagger_{q_n} + \hat{a}_{q_n}) + \sum_{n,q_n} \omega_{q_n} (\hat{a}^\dagger_{q_n} \hat{a}_{q_n} + 1/2) \tag{S1}$$

where $q_n$ is a harmonic oscillator in thermal bath $n$ with frequency $\omega_{q_n}$ and creation operator $\hat{a}_{q_n}$. Each oscillator is linearly coupled to the system by system-bath coupling operator $\hat{L}_n$ with a coupling strength $\Lambda_{q_n}$ described by the spectral density

$$J_n(\omega) = \pi \sum_{q_n} |\Lambda_{q_n}|^2 \delta(\omega - \omega_{q_n}). \tag{S2}$$

The statistical behavior of each bath is described by the time correlation function

$$C_n(t) = \frac{1}{\pi} \int_0^\infty d\omega J_n(\omega) \big( \coth(\frac{\beta\omega}{2}) \cos(\omega t/\hbar) - i \sin(\omega t/\hbar) \big) = \sum_{j_n} C_{j_n}(t) = \sum_{j_n} g_{j_n} e^{-\gamma_{j_n} t/\hbar} \tag{S3}$$

which is decomposed into a set of exponential modes, $j_n$.

Following the non-Markovian Quantum State Diffusion (NMQSD) formalism, HOPS uses a stochastic unraveling to produce an ensemble of noise trajectories $\mathbf{z}$, made up of terms $z_{n,t}$ indexed by bath $n$ and time $t$ and characterized by ensemble average ($\mathbb{E}_{\mathbf{z}}[\cdot]$) properties $\mathbb{E}_{\mathbf{z}}[z_{n,t}] = \mathbb{E}_{\mathbf{z}}[z_{n,t} z_{m,s}] = 0$ and $\mathbb{E}_{\mathbf{z}}[z^*_{n,t} z_{m,s}] = \delta_{m,n} C_n(t-s)$. Each noise trajectory is associated with the time-evolution of a system wave function $|\psi_t^{(\vec{0})}\rangle$.[3] While the time-evolution associated with a single noise trajectory does not correspond to a single instance of the system,[4] the reduced density matrix of the system at each point in time is given exactly by the ensemble average

$$\hat{\rho}_t = \mathbb{E}_{\mathbf{z}}[|\psi_t^{(\vec{0})}\rangle\langle\psi_t^{(\vec{0})}|] \tag{S4}$$

where $|\psi_t^{(\vec{0})}\rangle$ is implicitly indexed by the noise trajectory $z$.

The open quantum system for a single trajectory is described at each time $t$ in the shared basis $|\vec{k}, s\rangle \in \mathbb{A} \bigotimes \mathbb{S}$. $|\vec{k}\rangle \in \mathbb{A} = \sum_{n,j_n} k_{j_n} \vec{e}_{j_n}$ is an auxiliary indexing vector, where $\{\vec{e}_{j_n}\}$ is a set of mutually orthogonal indexing vectors that correspond to the exponential modes of each bath correlation function. The auxiliary basis, $\mathbb{A}$, is limited to a finite size by the introduction of a maximum hierarchy depth $k_{\max}$ such that $|\vec{k}\rangle \in \mathbb{A}$ if $0 \leq \sum_{n,j_n} k_{j_n} \leq k_{\max}$. $|s\rangle \in \mathbb{S}$ is system state, where the state basis $\mathbb{S}$ spans the Hilbert space of $\hat{H}_S$. The full HOPS wave function at $t$ is given

$$|\Psi_t\rangle = \sum_{\vec{k} \in \mathbb{A}_t} \sum_{s \in \mathbb{S}_t} \Psi[\vec{k}, s] |\vec{k}, s\rangle \tag{S5}$$

where $\mathbb{A}_t$ and $\mathbb{S}_t$ are the time-dependent adaptive auxiliary and state bases, respectively, which are subsets of the full auxiliary and state basis $\mathbb{A}$ and $\mathbb{S}$.

It is convenient to think of the full HOPS wave function as consisting of auxiliary wave functions represented in the state basis,

$$|\Psi_t\rangle = \sum_{\vec{k} \in \mathbb{A}_t} |\psi_t^{(\vec{k})}\rangle |\vec{k}\rangle \tag{S6}$$

where each auxiliary wave function represents a component of the non-Markovian bath memory.

## B. The HOPS Equation-of-Motion

The time-evolution of the HOPS wave function for a single trajectory is given by the time-derivative super-operator $\mathscr{L}_t$, such that

$$\partial_t |\Psi_t\rangle = \mathscr{L}_t |\Psi_t\rangle. \tag{S7}$$

The action of this super-operator is gvien by the normalized nonlinear HOPS equation-of-motion, which can be written in terms of the auxiliary wave functions:[1,2,5]

$$\begin{aligned}\hbar\frac{d|\psi_t^{(\vec{k})}\rangle}{dt} = \big(-i\hat{H}_S - \vec{k}\cdot\vec{\gamma} - \Gamma_t + \sum_n \hat{L}_n(z^*_{n,t} + \sum_{j_n}\xi_{j_n,t}) + \hat{T}\big)|\psi_t^{(\vec{k})}\rangle \\ + \sum_{n,j_n} k_{j_n}\gamma_{j_n}\hat{L}_n|\psi_t^{(\vec{k}-\vec{e}_{j_n})}\rangle \\ - \sum_{n,j_n}\Big(\frac{g_{j_n}}{\gamma_{j_n}}\Big)(\hat{L}_n^\dagger - \langle\hat{L}_n^\dagger\rangle_t)|\psi_t^{(\vec{k}+\vec{e}_{j_n})}\rangle.\end{aligned} \tag{S8}$$

where $z_{n,t}$ is the stochastic fluctuation, or noise, arising from the interaction of the system and the $n^{\text{th}}$ environment at time $t$,

$$\langle\hat{L}_n^\dagger\rangle_t = \langle\psi_t^{(\vec{0})}|\hat{L}_n^\dagger|\psi_t^{(\vec{0})}\rangle \tag{S9}$$

is the expectation value of the $n^{\text{th}}$ system-bath coupling operator,

$$\begin{aligned}\Gamma_t = & \sum_n \langle\hat{L}_n\rangle_t \,\mathrm{Re}[z^*_{n,t} + \sum_{j_n}\xi_{j_n,t}] \\ & - \sum_{n,j_n}\mathrm{Re}\Big[\Big(\frac{g_{j_n}}{\gamma_{j_n}}\Big)\langle\psi_t^{(\vec{0})}|\hat{L}_n^\dagger|\psi_t^{(\vec{e}_{j_n})}\rangle\Big] \\ & + \sum_{n,j_n}\langle\hat{L}_n^\dagger\rangle_t \,\mathrm{Re}\Big[\Big(\frac{g_{j_n}}{\gamma_{j_n}}\Big)\langle\psi_t^{(\vec{0})}|\psi_t^{(\vec{e}_{j_n})}\rangle\Big]\end{aligned} \tag{S10}$$

is a normalization correction factor[6],

$$\xi_{j_n,t} = \frac{1}{\hbar}\int_0^t d\tau C^*_{j_n}(t-\tau)\,\langle\hat{L}_n^\dagger\rangle_\tau \tag{S11}$$

is the noise memory drift term of correlation function mode $j_n$, and $\hat{T}$ is the low-temperature correction[5]

$$\begin{aligned}\hat{T}|\psi_t^{(\vec{k})}\rangle = \sum_n\Bigg(\Big(G_n^*\langle\hat{L}_n^\dagger\rangle_t + \delta_{\vec{k}=\vec{0}}(G_n\langle\hat{L}_n^\dagger\rangle_t - G_n\hat{L}_n^\dagger)\Big)\hat{L}_n|\psi_t^{(\vec{k})}\rangle \\ -\mathrm{Re}[G_n](2\langle\hat{L}_n^\dagger\rangle_t\langle\hat{L}_n\rangle_t - \langle\hat{L}_n^\dagger\hat{L}_n\rangle_t)|\psi_t^{(\vec{k})}\rangle\Bigg)\end{aligned} \tag{S12}$$

that accounts for the ultrafast correlation function modes $\{\nu_n\}$ of each bath $n$, which are excluded from the set $\{j_n\}$, where

$$G_n = \sum_{\nu_n}\frac{g_{\nu_n}}{\gamma_{\nu_n}}. \tag{S13}$$

The second line of $\hat{T}|\psi_t^{(\vec{k})}\rangle$ accounts for the low-temperature correction to the normalization correction factor $\Gamma_t$. When no low-temperature correction is included (which is true for all calculations presented here), $G_n = 0 \forall n \ni \hat{T} = 0$. Note that the equation-of-motion allows for direct fluxes between auxiliary basis members $|\vec{k}\rangle$ and $|\vec{k}\pm\vec{e}_{j_n}\rangle$ only.

### C. Redefinition of Terms

Throughout this derivation, we make reference to modes $m$ as a simpler-to-read replacement index for $j_n$, and $\hat{L}_n$, the system-bath projection operator for a bath containing mode $j_n = m$, is written $\hat{L}_m$. To reduce the difficulty of adaptive error calculations, we use a mode basis $\mathbb{M}_t$ to limit the number of correlation function modes $\{m\}$ to the relevant subset at each point in time. The mode basis is not calculated using an error bound, but rather is the list of all modes relevant to the current state and auxiliary bases: $m \ni \sum_{d \in \mathbb{S}} \sum_{s \in \mathbb{S}_t} |\hat{L}_m[d,s]| > 0$ or $m \ni \sum_{\vec{k} \in \mathbb{A}_t} |k_m| > 0$.

The only place this replacement index $m$ cannot be trivially applied is to the term

$$\sum_n \hat{L}_n (z^*_{n,t} + \sum_{j_n} \xi_{j_n,t}) \tag{S14}$$

so in the derivation below this term is included implicitly when the equation-of-motion is called, or by a noise matrix in the same Hilbert space as the system Hamiltonian,

$$\hat{Z}_t = \sum_n \hat{L}_n (z^*_{n,t} + \sum_{j_n} \xi_{j_n,t}). \tag{S15}$$

We refer to the sum $\hat{H}_S + \hat{Z}_t + \hat{T}$ as the augmented system Hamiltonian, and make reference to it in the main text.[7]

To account for the interconnected nature of the states and auxiliary indexing vectors under the action of the HOPS equation-of-motion, we introduce a set of ancillary bases by their relationship to the full and adaptive auxiliary and state bases below in Table 1.

| Basis | Description | Index | Mathematical description |
|---|---|---|---|
| $\mathbb{A}$ | The full auxiliary basis | $\vec{k}$ | $\lVert\vec{k}\rVert_1 \leq k_{\max}$ |
| $\mathbb{A}_t$ | The adaptive auxiliary basis at time $t$ | $\vec{k}$ | $\vec{k} \in \mathbb{A}_t$ |
| $\mathbb{A} \setminus \mathbb{A}_t$ | The compliment of the auxiliary basis at time $t$ | $\vec{k}_b$ | $\vec{k}_b \notin \mathbb{A}_t$ |
| $\mathbb{A}^s_{t+\Delta t}$ | The stable auxiliary basis at time $t+\Delta t$ | $\vec{k}$ | $\vec{k} \in \mathbb{A}_{t+\Delta t} \cap \mathbb{A}_t$ |
| $\mathbb{A}^b_{t+\Delta t}$ | The boundary auxiliary basis at time $t+\Delta t$ | $\vec{k}_b$ | $\vec{k}_b \in \mathbb{A}_{t+\Delta t} \cap (\mathbb{A} \setminus \mathbb{A}_t)$ |
| $\mathbb{S}$ | The full state basis | $s$ | $\hat{H}_S \lvert s\rangle$ is defined |
| $\mathbb{S}_t$ | The adaptive state basis at time $t$ | $s$ | $s \in \mathbb{S}_t$ |
| $\mathbb{S} \setminus \mathbb{S}_t$ | The compliment of the state basis at time $t$ | $s_b$ | $s_b \notin \mathbb{S}_t$ |
| $\mathbb{S}^s_{t+\Delta t}$ | The stable state basis at time $t+\Delta t$ | $s$ | $s \in \mathbb{S}_{t+\Delta t} \cap \mathbb{S}_t$ |
| $\mathbb{S}^b_{t+\Delta t}$ | The boundary state basis at time $t+\Delta t$ | $s_b$ | $s_b \in \mathbb{S}_{t+\Delta t} \cap (\mathbb{S} \setminus \mathbb{S}_t)$ |
| $\mathbb{S}^d_t$ | The destination state basis at time $t$ | $d$ | $\lvert \sum_{m \in \mathbb{M}_t} \sum_{s \in \mathbb{S}_t} \hat{L}_m[d,s] \rvert > 0$ |
| $\mathbb{M}_t$ | The mode basis at time $t$ | $m$ | $\lvert \langle \hat{L}_m \rangle_t \rvert + \lvert \sum_{\vec{k} \in \mathbb{A}_t} \vec{k}[m] \rvert > 0$ |

TABLE S1. The bases and their elements. Note that $\mathbb{A}_t$ and $\mathbb{S}_t$ are directly defined by the adaptive algorithm, while other bases are defined based on $\mathbb{A}_t$ and $\mathbb{S}_t$.

#### D. The Adaptive Algorithm

The core of adHOPS is the use of a subset of the full auxiliary and state bases $\mathbb{A}_t$ and $\mathbb{S}_t$ to represent and time-evolve the HOPS wave function. Because of the sparsity in the HOPS wave function induced by dynamic localization and the locality of connections between basis elements (connections only exist between neighboring auxiliary wave functions by the definition of the equation-of-motion and relatively proximate electronic states by the parameters of molecular materials), the relevant portions of each basis are much smaller than the full set in extended systems. At each point in time (or every $u_t$ fs, if using an adaptive update step)[5], an adHOPS calculation generates a new auxiliary and state basis, $\mathbb{A}_{t+\Delta t}$ and $\mathbb{S}_{t+\Delta t}$, prior to time-evolution. We set a bound on the derivative error introduced by the change of the adaptive basis:

$$E^2 = \left\| \frac{d|\Psi_t\rangle}{dt} - \frac{d|\hat{\Psi}_t\rangle}{dt} \right\|_2^2 \leq \delta_A^2 + \delta_S^2 \tag{S16}$$

where $|\Psi_t\rangle$ is the HOPS wave function at time $t$ in the full basis $\mathbb{A} \bigotimes \mathbb{S}$, $|\hat{\Psi}\rangle$ is the same HOPS wave function truncated to the reduced basis $\mathbb{A}_{t+\Delta t} \bigotimes \mathbb{S}_{t+\Delta t}$, and $\delta_A$ and $\delta_S$ are user-defined error bounds. Note that while $|\Psi_t\rangle$ exists in the full basis, in practice it is populated only in the reduced basis determined during the previous time step, $\mathbb{A}_t \bigotimes \mathbb{S}_t$, and the corresponding time-derivative

$$\frac{d|\Psi_t\rangle}{dt} = \sum_{\vec{k} \in \mathbb{A}} \sum_{s \in \mathbb{S}} \frac{d\Psi[\vec{k},s]}{dt} |\vec{k},s\rangle \tag{S17}$$

is 0 for all $\vec{k}$ that do not satisfy either $\vec{k} \in \mathbb{A}_t$ or $\vec{k} \pm e_m \in \mathbb{A}_t$ for some $m \in \mathbb{M}_t$, and for all $s$ that do not satisfy either $s \in \mathbb{S}_t$, $s \in \mathbb{S}_t^d$, or $\sum_{s' \in \mathbb{S}_t} |\hat{H}_S[s',s]| > 0$.

Noting that auxiliaries are only connected to those one step up or down along a single mode, we can write Eq. (S7) as

$$\begin{aligned} \frac{d\Psi_t[\vec{k},d]}{dt} =& \sum_s \mathscr{L}[\vec{k},d,\vec{k},s]\Psi_t[\vec{k},s] \\ &+ \sum_m \sum_s \mathscr{L}[\vec{k},d,\vec{k}+\vec{e}_m,s]\Psi_t[\vec{k}+\vec{e}_m,s] \\ &+ \sum_m \sum_s \mathscr{L}[\vec{k},d,\vec{k}-\vec{e}_m,s]\Psi_t[\vec{k}-\vec{e}_m,s] \end{aligned} \tag{S18}$$

where the first term on the right-hand side represents the transitions between states within a single auxiliary wave function, stemming from the system Hamiltonian, noise, etc., and the second and third terms on the right-hand side represent fluxes from auxiliary wave functions one step higher or lower in the hierarchy, respectively.

The calculation of an auxiliary basis that satisfies the error bounds is confounded by the presence of flux terms between previously-populated auxiliary vectors removed during the construction of $\mathbb{A}_{t+\Delta t}$. Determining a minimum auxiliary basis that satisfies the derivative error bound $\delta_A$ would involve calculating the derivative error associated with each combination of deleted auxiliary vectors, which is computationally impractical. Thus, we calculate the derivative error associated with neglecting each auxiliary vector individually. We calculate the derivative error associated with neglecting individual states in the same manner. We define $E_{\mathbb{A}_t^s}[\vec{k}]$ and $E_{\mathbb{S}_t^s}[s]$ as the derivative errors arising from removing auxiliary vector $|\vec{k}\rangle \in \mathbb{A}_t$ and state $s \in \mathbb{S}_t$ when integrating from $t \to t+\Delta t$. The derivative errors from continuing to neglect auxiliary vector $|\vec{k}_b\rangle \in \mathbb{A} \setminus \mathbb{A}_t$ and state $|s_b\rangle \in \mathbb{S} \setminus \mathbb{S}_t$ are $E_{\mathbb{A}_t^b}[\vec{k}_b]$ and $E_{\mathbb{S}_t^b}[s_b]$, respectively. We find an upper bound on the derivative error - that is, the 2-norm difference between $\frac{d|\tilde{\Psi}_t\rangle}{dt}$, the time-derivative of the adHOPS wave function at time $t$ (projected into the full basis $\mathbb{A} \bigotimes \mathbb{S}$ to ensure derivative terms that leave the basis $\mathbb{A}_t \bigotimes \mathbb{S}_t$ are not ignored), and $\frac{d|\hat{\Psi}_t\rangle}{dt}$, the time-derivative limited to some trial basis $\mathbb{A}_{t+\Delta t} \bigotimes \mathbb{S}_{t+\Delta t}$:

$$\begin{aligned} \left\| \frac{d|\tilde{\Psi}_t\rangle}{dt} - \frac{d|\hat{\Psi}_t\rangle}{dt} \right\|_2^2 \leq& \sum_{\vec{k} \in \mathbb{A}_t \setminus \mathbb{A}_{t+\Delta t}} E^2_{\mathbb{A}_t^s}[\vec{k}] + \sum_{\vec{k}_b \in \mathbb{A} \setminus (\mathbb{A}_t \cup \mathbb{A}_{t+\Delta t})} E^2_{\mathbb{A}_t^b}[\vec{k}_b] \\ &+ \sum_{s \in \mathbb{S}_t \setminus \mathbb{S}_{t+\Delta t}} E^2_{\mathbb{S}_t^s}[s] + \sum_{s_b \in \mathbb{S} \setminus (\mathbb{S}_t \cup \mathbb{S}_{t+\Delta t})} E^2_{\mathbb{S}_t^b}[s_b] \end{aligned} \tag{S19}$$

which in turn must satisfy derivative error bound $\delta^2 = \delta_S^2 + \delta_A^2$ by conditions

$$\sum_{\vec{k} \in \mathbb{A}_t \setminus \mathbb{A}_{t+\Delta t}} E^2_{\mathbb{A}_t^s}[\vec{k}] + \sum_{\vec{k}_b \in \mathbb{A} \setminus (\mathbb{A}_t \cup \mathbb{A}_{t+\Delta t})} E^2_{\mathbb{A}_t^b}[\vec{k}_b] \leq \delta_A^2 \tag{S20}$$

and

$$\sum_{s \in \mathbb{S}_t \setminus \mathbb{S}_{t+\Delta t}} E^2_{\mathbb{S}_t^s}[s] + \sum_{s_b \in \mathbb{S} \setminus (\mathbb{S}_t \cup \mathbb{S}_{t+\Delta t})} E^2_{\mathbb{S}_t^b}[s_b] \leq \delta_S^2. \tag{S21}$$

For each of the four groups of errors, we find a reduced basis by removing the maximum number of elements guaranteed not to violate the associated error bound. To do this, we sort the errors of a given group from smallest to largest and discard as many elements as possible, in ascending order of introduced error, while satisfying the error bound.

In both the auxiliary and state basis cases, the stable elements are analyzed and removed before the boundary elements. To ensure a relatively even distribution of error between the stable and boundary sub-bases, we remove the maximum number of stable $|\vec{k}\rangle$ such that

$$\sum_{\vec{k} \in \mathbb{A}_t \setminus \mathbb{A}_{t+\Delta t}} E^2_{\mathbb{A}_t^s}[\vec{k}] = E^2_{\mathbb{A}_t^s} \leq \frac{\delta_A^2}{2} \tag{S22}$$

then the maximum number of boundary $|\vec{k}_b\rangle$ such that

$$\sum_{\vec{k}_b \in \mathbb{A} \setminus (\mathbb{A}_t \cup \mathbb{A}_{t+\Delta t})} E^2_{\mathbb{A}_t^b}[\vec{k}_b] = E^2_{\mathbb{A}_t^b} \leq \delta_A^2 - E^2_{\mathbb{A}_t^s}. \tag{S23}$$

Similarly, the stable $|s\rangle$ are removed to maximize

$$\sum_{s \in \mathbb{S}_t \setminus \mathbb{S}_{t+\Delta t}} E^2_{\mathbb{S}_t^s}[s] = E^2_{\mathbb{S}_t^s} \leq \frac{\delta_S^2}{2} \tag{S24}$$

within the bound before the boundary $|s_b\rangle$ are removed to satisfy

$$\sum_{s_b \in \mathbb{S} \setminus (\mathbb{S}_t \cup \mathbb{S}_{t+\Delta t})} E^2_{\mathbb{S}_t^b}[s_b] = E^2_{\mathbb{S}_t^b} \leq \delta_S^2 - E^2_{\mathbb{S}_t^s}. \tag{S25}$$

Thus, we calculate each of these four sets of error terms in sequence, as detailed below.

## S2. ERROR CALCULATIONS

In this section, we explicitly find the error associated with excluding each basis element in the four groups enumerated above. Use of the $\leq$ symbol indicates that error is calculated in a manner that finds an upper bound on an error term greater than those derived in previous lines: that is, some possibility of destructive interference that limits flux is ignored. Thus, the actual derivative error $\left\| \frac{d|\tilde{\Psi}_t\rangle}{dt} - \frac{d|\hat{\Psi}_t\rangle}{dt} \right\|_2^2 \leq \delta$.

In this section, we use the following terms: $\vec{k}$ is an auxiliary indexing vector in the current basis. Conversely, $\vec{k}_b$ is an auxiliary indexing vector not in the current basis. Likewise, $s$ and $s_b$ are states in and not in the current basis, respectively. Finally, $d$ is a destination state that accepts flux from some state $s$ and might belong to either the set of $\{s\}$ or the set of $\{s_b\}$. Much like the mode basis, we define a basis of destination states, $\mathbb{S}_t^d$, by $d \in \mathbb{S}_t^d$ if $\sum_m \sum_{s \in \mathbb{S}_t} |\hat{L}_m[d,s]| > 0$.

For reasons that will become clear in the state basis section, we split $\hat{L}_m$ into diagonal and off-diagonal components (in terms of the Hilbert space of $\hat{H}_S$). For convenience, we define the matrices

$$M^{diag}[m,s] = \hat{L}_m[s,s] \tag{S26}$$

$$M_d^{off}[m,s] = \hat{L}_m[d,s](1 - \delta_{d,s}) \tag{S27}$$

and

$$X[m,s] = \langle \hat{L}_m \rangle_t. \tag{S28}$$

In each of these matrices, rows correspond to modes $m \in \mathbb{M}_t$, and columns to states in $|s\rangle \in \mathbb{S}_t$.

To illustrate the separation of $\hat{L}_m$, take the example of a system with 2 total correlation function modes and 3 states in the system Hilbert space. The first mode is associated with

$$\hat{L}_a = 2|1\rangle\langle 1| + i|1\rangle\langle 2| - i|2\rangle\langle 1| + |2\rangle\langle 2| = \begin{bmatrix} 2 & i & 0 \\ -i & 1 & 0 \\ 0 & 0 & 0 \end{bmatrix} \tag{S29}$$

and the second with

$$\hat{L}_b = |2\rangle\langle 3| + |3\rangle\langle 2| - |3\rangle\langle 3| = \begin{bmatrix} 0 & 0 & 0 \\ 0 & 0 & 1 \\ 0 & 1 & -1 \end{bmatrix}. \tag{S30}$$

We would find that

$$M^{diag} = \begin{bmatrix} 2 & 1 & 0 \\ 0 & 0 & -1 \end{bmatrix} \tag{S31}$$

$$M_1^{off} = \begin{bmatrix} 0 & i & 0 \\ 0 & 0 & 0 \end{bmatrix}, \quad M_2^{off} = \begin{bmatrix} -i & 0 & 0 \\ 0 & 0 & 1 \end{bmatrix}, \quad M_3^{off} = \begin{bmatrix} 0 & 0 & 0 \\ 0 & 1 & 0 \end{bmatrix} \tag{S32}$$

and

$$X = \begin{bmatrix} \langle \hat{L}_a \rangle_t & \langle \hat{L}_a \rangle_t & \langle \hat{L}_a \rangle_t \\ \langle \hat{L}_b \rangle_t & \langle \hat{L}_b \rangle_t & \langle \hat{L}_b \rangle_t \end{bmatrix}. \tag{S33}$$

The matrix form of the error calculations presented here reflects the implementation of the derivative error calculations in MesoHOPS v1.6.

### A. Adaptive Auxiliary Basis

The derivative error introduced by excluding $|\vec{k}\rangle \in \mathbb{A}$ from the auxiliary basis $\mathbb{A}_{t+\Delta t}$ is given by

$$\begin{aligned} E^2_{\mathbb{A}_t}[\vec{k}] = &\sum_{s \in \mathbb{S}_t} \left| \left(\mathscr{L}_{\mathbb{A}_t \otimes \mathbb{S}_t} \Psi_t\right)[\vec{k},s] + \frac{\Psi_t[\vec{k},s]}{\Delta t} \right|^2 \\ &+ \sum_m \sum_{s \in \mathbb{S}_t} \left| \mathscr{L}[\vec{k}+\vec{e}_m, s, \vec{k}, s] \Psi_t[\vec{k},s] \right|^2 \\ &+ \sum_{d \neq s \in \mathbb{S}_t^d} \sum_m \left| \sum_{s \in \mathbb{S}_t} \mathscr{L}[\vec{k}+\vec{e}_m, d, \vec{k}, s] \Psi_t[\vec{k},s] \right|^2 \\ &+ \sum_m \sum_{s \in \mathbb{S}_t} \left| \mathscr{L}[\vec{k}-\vec{e}_m, s, \vec{k}, s] \Psi_t[\vec{k},s] \right|^2 \\ &+ \sum_{d \neq s \in \mathbb{S}_t^d} \sum_m \left| \sum_{s \in \mathbb{S}_t} \mathscr{L}[\vec{k}-\vec{e}_m, d, \vec{k}, s] \Psi_t[\vec{k},s] \right|^2 \\ &+ \sum_{s_b \in \mathbb{S} \setminus \mathbb{S}_t} \left| \sum_{s \in \mathbb{S}_t} \mathscr{L}[\vec{k}, s_b, \vec{k}, s] \Psi_t[\vec{k},s] \right|^2. \end{aligned} \tag{S34}$$

The first term is the squared error arising from the flux into $|\psi_t^{(\vec{k})}\rangle$ constructed as the sum of the flux when the equation-of-motion is restricted to the basis $\mathbb{A}_t \otimes \mathbb{S}_t$ ($\mathscr{L}_{\mathbb{A}_t \otimes \mathbb{S}_t}|\Psi_t\rangle$) and the deletion flux ($\Psi_t[\vec{k},s]/\Delta t$) that is implicitly added to the time-evolution to account for $|\psi_t^{(\vec{k})}\rangle \rightarrow 0$ when $|\vec{k}\rangle$ is removed from the basis (where $\Delta t$ is the integration time step). The second and third (fourth and fifth) terms are the squared errors arising from flux up (down) into neighboring auxiliary wave functions $|\psi_t^{(\vec{k}')}\rangle$ for $|\vec{k}'\rangle = |\vec{k} \pm \vec{e}_m\rangle \in \mathbb{A}$. Note that these terms account for the diagonal flux (from source state $|s\rangle$ to the same state) and the off-diagonal flux (to destination states $|d\rangle \neq |s\rangle$) separately. Finally, the sixth term only includes contribution from populated states $|s\rangle$ to unpopulated states $|s_b\rangle$ in the auxiliary wave function $|\psi_t^{(\vec{k})}\rangle$ arising from couplings within the augmented system Hamiltonian (i.e., $|\vec{k},s\rangle \rightarrow |\vec{k},s_b\rangle$ when $|s\rangle \in \mathbb{S}_t$ and $|s_b\rangle \in \mathbb{S} \setminus \mathbb{S}_t$), because all other fluxes of this form are either 0 or were included in the first term.

Expanding the terms in Eq. (S34) using the normalized nonlinear HOPS equation (Eq. (S8)) and combining lines 2 and 3 and lines 4 and 5, the squared derivative error from excluding $|\vec{k}\rangle$ becomes

$$\begin{aligned} E^2_{\mathbb{A}_t}[\vec{k}] = &\sum_{s\in\mathbb{S}_t}\left|\left(\mathscr{L}_{\mathbb{A}_t\otimes\mathbb{S}_t}\Psi_t\right)[\vec{k},s] + \frac{\Psi_t[\vec{k},s]}{\Delta t}\right|^2 \\ &+ \frac{1}{\hbar^2}\sum_{d\in\mathbb{S}_t^d}\sum_{m:\vec{k}+\vec{e}_m\in\mathbb{A}}\left|\sum_{s\in\mathbb{S}_t}(k_m+1)\gamma_m\hat{L}_m[d,s]\Psi_t[\vec{k},s]\right|^2 \\ &+ \frac{1}{\hbar^2}\sum_{d\in\mathbb{S}_t^d\cup\mathbb{S}_t}\sum_{m:\vec{k}-\vec{e}_m\in\mathbb{A}}\left|\sum_{s\in\mathbb{S}_t}\frac{g_m}{\gamma_m}(\hat{L}_m[d,s]-\langle\hat{L}_m\rangle_t\,\delta_{d,s})\Psi_t[\vec{k},s]\right|^2 \\ &+ \frac{1}{\hbar^2}\sum_{s_b\in\mathbb{S}\setminus\mathbb{S}_t}\left|\sum_{s\in\mathbb{S}_t}\left(-i\hat{H}_S+\hat{Z}_t+\hat{T}^{(\vec{k})}\right)[s_b,s]\Psi_t[\vec{k},s]\right|^2 \end{aligned} \tag{S35}$$

We note that the numerical construction of $(\mathscr{L}_{\mathbb{A}_t\otimes\mathbb{S}_t}|\Psi_t\rangle)$is performed as an additional derivative evaluation using the HOPS equation expressed in the reduced basis $\mathbb{A}_t\otimes\mathbb{S}_t$. The $\delta_{d,s}$ term in the third line stems from the fact that a scalar added to a matrix is implicitly multiplied by the identity.

### *1. Stable Auxiliary Basis*

Starting from Eq. (S35), we explicitly calculate the error contributions associated with excluding $|\vec{k}\rangle \in \mathbb{A}_t$ from the basis $\mathbb{A}_{t+\Delta t}$ as described below. The two components of the flux-in error calculation,

$$E^2_{\mathbb{A}_t^s,\mathrm{in}}[\vec{k},s] = \left|\left(\mathscr{L}_{\mathbb{A}_t\otimes\mathbb{S}_t}\Psi_t\right)[\vec{k},s] + \frac{\Psi_t[\vec{k},s]}{\Delta t}\right|^2 \tag{S36}$$

are calculated together because they contribute to the same amplitudes and, as a result, may exhibit cancellations.

The flux-up error calculation,

$$\begin{aligned} \hbar^2 E^2_{\mathbb{A}_t^s,\mathrm{up}}[\vec{k},m] &= \sum_{d\in\mathbb{S}_t^d}\delta_{\vec{k}+\vec{e}_m\in\mathbb{A}}\left|\sum_{s\in\mathbb{S}_t}(k_m+1)\gamma_m\hat{L}_m[d,s]\Psi_t[\vec{k},s]\right|^2 \\ &= F_{\mathbb{A}_t^s,\mathrm{up}}[\vec{k},m]|(k_m+1)\gamma_m|^2\sum_{d\in\mathbb{S}_t^d}\left|\sum_{s\in\mathbb{S}_t}\hat{L}_m[d,s]\Psi_t[\vec{k},s]\right|^2 \\ &\le F_{\mathbb{A}_t^s,\mathrm{up}}[\vec{k},m]|(k_m+1)\gamma_m|^2\sum_{d\in\mathbb{S}_t^d}\sum_{s\in\mathbb{S}_t}\left|\hat{L}_m[d,s]\Psi_t[\vec{k},s]\right|^2 \\ &= F_{\mathbb{A}_t^s,\mathrm{up}}[\vec{k},m]|(k_m+1)\gamma_m|^2\sum_{s\in\mathbb{S}_t}\left|\Psi_t[\vec{k},s]\right|^2\sum_{d\in\mathbb{S}_t^d}\left|\hat{L}_m[d,s]\right|^2 \\ &= F_{\mathbb{A}_t^s,\mathrm{up}}[\vec{k},m]|(k_m+1)\gamma_m|^2\sum_{s\in\mathbb{S}_t}\left|\Psi_t[\vec{k},s]\right|^2\sum_{d\in\mathbb{S}_t^d}\left|M^{diag}[m,s]\delta_{d,s}+M_d^{off}[m,s]\right|^2 \\ &= F_{\mathbb{A}_t^s,\mathrm{up}}[\vec{k},m]|(k_m+1)\gamma_m|^2\sum_{s\in\mathbb{S}_t}\left|\Psi_t[\vec{k},s]\right|^2\left(\left|M^{diag}\right|^2+\sum_{d\in\mathbb{S}_t^d}\left|M_d^{off}\right|^2\right)[m,s] \end{aligned} \tag{S37}$$

is simplified by introducing $F_{\mathbb{A}_t^s,\mathrm{up}}[\vec{k},m] = \delta_{\vec{k}+\vec{e}_m\in\mathbb{A}}$, a filter restricting the sum over modes to only include fluxes to valid auxiliary vectors. In the final step, we may split up the absolute-squared sum of the diagonal and off-diagonal $M$ matrices because, by construction, $M_d^{off}[m,d] = 0$.

We retain error terms prior to applying the filter as $\tilde{E}^2_{\mathbb{A}_t^s,\mathrm{up}}[\vec{k},m]$, such that

$$E^2_{\mathbb{A}_t^s,\mathrm{up}}[\vec{k},m] = F_{\mathbb{A}_t^s,\mathrm{up}}[\vec{k},m]\tilde{E}^2_{\mathbb{A}_t^s,\mathrm{up}}[\vec{k},m]. \tag{S38}$$

This unfiltered error matrix is used below in error calculations for the boundary auxiliary basis.

The flux-down error calculation is given by

$$\begin{aligned}
\hbar^2 E^2_{\mathbb{A}^s_t,\text{down}}[\vec{k},m] &= \sum_{d\in\mathbb{S}^d_t\cup\mathbb{S}_t} \delta_{\vec{k}-\vec{e}_m\in\mathbb{A}} \left|\sum_{s\in\mathbb{S}_t}\frac{g_m}{\gamma_m}(\hat{L}_m[d,s]-\langle\hat{L}_m\rangle_t\,\delta_{d,s})\Psi_t[\vec{k},s]\right|^2 \\
&= F_{\mathbb{A}^s_t,\text{down}}[\vec{k},m]\left|\frac{g_m}{\gamma_m}\right|^2 \sum_{d\in\mathbb{S}^d_t\cup\mathbb{S}_t}\left|\sum_{s\in\mathbb{S}_t}(\hat{L}_m[d,s]-\langle\hat{L}_m\rangle_t\,\delta_{d,s})\Psi_t[\vec{k},s]\right|^2 \\
&\leq F_{\mathbb{A}^s_t,\text{down}}[\vec{k},m]\left|\frac{g_m}{\gamma_m}\right|^2 \sum_{d\in\mathbb{S}^d_t\cup\mathbb{S}_t}\sum_{s\in\mathbb{S}_t}\left|(\hat{L}_m[d,s]-\langle\hat{L}_m\rangle_t\,\delta_{d,s})\Psi_t[\vec{k},s]\right|^2 \\
&= F_{\mathbb{A}^s_t,\text{down}}[\vec{k},m]\left|\frac{g_m}{\gamma_m}\right|^2 \sum_{s\in\mathbb{S}_t}\left|\Psi_t[\vec{k},s]\right|^2 \sum_{d\in\mathbb{S}^d_t\cup\mathbb{S}_t}\left|(\hat{L}_m[d,s]-\langle\hat{L}_m\rangle_t\,\delta_{d,s})\right|^2 \\
&= F_{\mathbb{A}^s_t,\text{down}}[\vec{k},m]\left|\frac{g_m}{\gamma_m}\right|^2 \sum_{s\in\mathbb{S}_t}\left|\Psi_t[\vec{k},s]\right|^2 \sum_{d\in\mathbb{S}^d_t\cup\mathbb{S}_t}\left|(M^{diag}-X)[m,s]\delta_{d,s}+M^{off}_d[m,s]\right|^2 \\
&= F_{\mathbb{A}^s_t,\text{down}}[\vec{k},m]\left|\frac{g_m}{\gamma_m}\right|^2 \sum_{s\in\mathbb{S}_t}\left|\Psi_t[\vec{k},s]\right|^2 \left(\left|(M^{diag}-X)\right|^2+\sum_{d\in\mathbb{S}^d_t}\left|M^{off}_d\right|^2\right)[m,s]
\end{aligned}\tag{S39}$$

and similarly simplified by introducing filter $F_{\mathbb{A}^s_t,\text{down}}[\vec{k},m]=\delta_{\vec{k}-\vec{e}_m\in\mathbb{A}}$. In the final step, we again take advantage of $M^{off}_d[m,d]=0$. As in the flux-up case, we retain the unfiltered error terms $\tilde{E}^2_{\mathbb{A}^s_t,\text{down}}[\vec{k},m]$, where

$$E^2_{\mathbb{A}^s_t,\text{down}}[\vec{k},m]=F_{\mathbb{A}^s_t,\text{down}}[\vec{k},m]\tilde{E}^2_{\mathbb{A}^s_t,\text{down}}[\vec{k},m]. \tag{S40}$$

Finally, the state-flux error calculation,

$$\begin{aligned}
\hbar^2 E^2_{\mathbb{A}^s_t,\text{state}}[\vec{k}] &= \sum_{s_b\in\mathbb{S}\setminus\mathbb{S}_t}\left|\sum_{s\in\mathbb{S}_t}\left(-i\hat{H}_S+\hat{Z}_t+\hat{T}^{(\vec{k})}\right)[s_b,s]\Psi_t[\vec{k},s]\right|^2 \\
&= \sum_{s_b\in\mathbb{S}\setminus\mathbb{S}_t}\left|\left(\left(-i\hat{H}_S+\hat{Z}_t+\hat{T}^{(\vec{k})}\right)\psi^{(\vec{k})}_t\right)[s_b]\right|^2
\end{aligned}\tag{S41}$$

evaluates the flux from populated states in auxiliary wave function $|\psi^{(\vec{k})}_t\rangle$ to states outside of the current basis $\mathbb{S}_t$. The total squared derivative error (S35) is

$$\begin{aligned}
E^2_{\mathbb{A}^s_t}[\vec{k}] = &\sum_{s\in\mathbb{S}_t} E^2_{\mathbb{A}^s_t,\text{in}}[\vec{k},s] \\
&+\sum_m E^2_{\mathbb{A}^s_t,\text{up}}[\vec{k},m] \\
&+\sum_m E^2_{\mathbb{A}^s_t,\text{down}}[\vec{k},m] \\
&+E^2_{\mathbb{A}^s_t,\text{state}}[\vec{k}].
\end{aligned}\tag{S42}$$

### *2. Boundary Auxiliary Basis*

Starting from Eq. (S35), the derivative error associated with excluding auxiliary vector ($|\vec{k}_b\rangle\in\mathbb{A}\setminus\mathbb{A}_t$) from $\mathbb{A}_{t+\Delta t}$ is only the sum of flux-up and flux-down terms arising from neighboring populated auxiliary wave functions (i.e., $|\psi^{(\vec{k})}_t\rangle\rightarrow|\psi^{(\vec{k}_b)}_t\rangle$ for $\vec{k}\in\mathbb{A}_t$), because $|\vec{k}_b\rangle$ is unpopulated. Note that flux into $|\vec{k}_b\rangle$ from the auxiliary vectors removed while constructing the stable auxiliary basis, $|\vec{k}\rangle\notin\mathbb{A}^s_{t+\Delta t}=\mathbb{A}_t\cap\mathbb{A}_{t+\Delta t}$, can be ignored because we have already accounted for the error associated with neglecting all fluxes from the auxiliary wave functions that have been deleted [Note: terminology]. As a result, we re-use the unfiltered versions of the (upper-bounded) flux-up and

flux-down squared error components constructed in Eqs. (S37) and (S39) with new filter functions, such that the squared derivative error associated with excluding $|\vec{k}_b\rangle \in \mathbb{A} \setminus \mathbb{A}_t$ from $\mathbb{A}_{t+\Delta t}$ is given by

$$E^2_{\mathbb{A}_t^b}[\vec{k}_b] = \sum_{m,\vec{k}:\vec{k}+\vec{e}_m=\vec{k}_b} F_{\mathbb{A}_t^b,\text{up}}[\vec{k},m]\tilde{E}^2_{\mathbb{A}_t^s,\text{up}}[\vec{k},m] + \sum_{m,\vec{k}:\vec{k}-\vec{e}_m=\vec{k}_b} F_{\mathbb{A}_t^b,\text{down}}[\vec{k},m]\tilde{E}^2_{\mathbb{A}_t^s,\text{down}}[\vec{k},m]. \tag{S43}$$

where $F_{\mathbb{A}_t^b,\text{up}} = \delta_{\vec{k}+\vec{e}_m \in \mathbb{A}\setminus\mathbb{A}_t}\delta_{\vec{k}\in\mathbb{A}^s_{t+\Delta t}}$ and $F_{\mathbb{A}_t^b,\text{down}} = \delta_{\vec{k}-\vec{e}_m \in \mathbb{A}\setminus\mathbb{A}_t}\delta_{\vec{k}\in\mathbb{A}^s_{t+\Delta t}}$.

## B. Adaptive State Basis

The derivative error for excluding $|s\rangle \in \mathbb{S}$ from $\mathbb{S}_{t+\Delta t}$ is the sum of errors associated with fluxes into and out of the state $s$ among all auxiliary wave functions. Since we use the auxiliary basis $\mathbb{A}_{t+\Delta t}$ during the construction of the state basis, it is convenient to define two kinds of basis elements: first, the stable auxiliary vectors ($|\vec{k}\rangle \in \mathbb{A}^s_{t+\Delta t} = \mathbb{A}_t \cap \mathbb{A}_{t+\Delta t}$) consisting of all auxiliary vectors that carried over from $\mathbb{A}_t$, and, second, the boundary auxiliary vectors newly added to the basis ($|\vec{k}_b\rangle \in \mathbb{A}^b_{t+\Delta t} = \mathbb{A}_{t+\Delta t} \setminus \mathbb{A}_t$). Taking into account this partitioning, the squared derivative error associated with excluding $|s\rangle$ from $\mathbb{S}_{t+\Delta t}$ is given as

$$\begin{aligned}
E^2_{\mathbb{S}_t}[s] = \sum_{\vec{k}\in\mathbb{A}^s_{t+\Delta t}} \Bigg( & \left| (\mathscr{L}_{\mathbb{A}^s_{t+\Delta t}\otimes\mathbb{S}_t}\Psi_t)[\vec{k},s] + \frac{\Psi_t[\vec{k},s]}{\Delta t} \right|^2 \\
& + \sum_{m:\vec{k}+\vec{e}_m\in\mathbb{A}^b_{t+\Delta t}} \left| \mathscr{L}[\vec{k}+\vec{e}_m,s,\vec{k},s]\Psi_t[\vec{k},s] \right|^2 \\
& + \sum_{m:\vec{k}+\vec{e}_m\in\mathbb{A}_{t+\Delta t}} \sum_{d\in\mathbb{S}^d_t\setminus\{s\}} \left| \mathscr{L}[\vec{k}+\vec{e}_m,d,\vec{k},s]\Psi_t[\vec{k},s] \right|^2 \\
& + \sum_{m:\vec{k}-\vec{e}_m\in\mathbb{A}^b_{t+\Delta t}} \left| \mathscr{L}[\vec{k}-\vec{e}_m,s,\vec{k},s]\Psi_t[\vec{k},s] \right|^2 \\
& + \sum_{m:\vec{k}-\vec{e}_m\in\mathbb{A}_{t+\Delta t}} \sum_{d\in\mathbb{S}^d_t\setminus\{s\}} \left| \mathscr{L}[\vec{k}-\vec{e}_m,d,\vec{k},s]\Psi_t[\vec{k},s] \right|^2 \\
& + \sum_{s'\in\mathbb{S}\setminus\{s\}} \left| \mathscr{L}[\vec{k},s',\vec{k},s]\Psi_t[\vec{k},s] \right|^2 \Bigg).
\end{aligned} \tag{S44}$$

The outer sum is restricted to $|\vec{k}\rangle \in \mathbb{A}^s_{t+\Delta t}$ because only stable auxiliary vectors can contribute non-zero flux. The first term contains the flux into state $|s\rangle$ constructed as a sum over the flux when the equation-of-motion is restricted to the basis $\mathbb{A}^s_{t+\Delta t}\otimes\mathbb{S}_t$ ($\mathscr{L}_{\mathbb{A}^s_{t+\Delta t}\otimes\mathbb{S}_t}|\Psi_t\rangle$) and the deletion flux ($\Psi_t[\vec{k},s]/\Delta t$) that is implicitly added to the time-evolution to account for all $\Psi_t[\vec{k},s] \to 0$ when $|s\rangle$ is removed from the basis (where $\Delta t$ is the integration time step). The second, third, fourth, and fifth terms are the squared errors arising from fluxes up and down. These fluxes are generally restricted to only flux into $|\vec{k}\rangle \in \mathbb{A}_{t+\Delta t}$: after all, the derivative error arising from neglecting flux into $|\psi_t^{(\vec{k}')}\rangle$ for $|\vec{k}'\rangle \in \mathbb{A}\setminus\mathbb{A}_{t+\Delta t}$ has already been accounted for during the calculation of $\mathbb{A}_{t+\Delta t}$. Furthermore, flux up or down from state $|s\rangle$ into the same state is restricted to fluxes into boundary auxiliary wave function $|\psi_t^{(\vec{k}_b)}\rangle$ for $|\vec{k}_b\rangle = |\vec{k}\pm\vec{e}_m\rangle \in \mathbb{A}^b_{t+\Delta t}$, because flux into the stable auxiliary wave functions is contained in the first term of Eq. (S44) (note that including the derivative flux in of these boundary auxiliary wave functions in the first term would double-count the associated error). Finally, the sixth term accounts for all flux out of the state $|s\rangle$ due to couplings in the augmented system Hamiltonian.

Expanding the terms in Eq. (S44) using the HOPS equation-of-motion (Eq. (S8)), the squared derivative error associated with excluding

state $|s\rangle \in \mathbb{S}$ from $\mathbb{S}_{t+\Delta t}$ is

$$
\begin{aligned}
E^2_{\mathbb{S}^s_t}[s] = &\sum_{\vec{k}\in\mathbb{A}^s_{t+\Delta t}} \left| (\mathscr{L}_{\mathbb{A}^s_{t+\Delta t}\otimes\mathbb{S}_t}\Psi_t)[\vec{k},s] + \frac{\Psi_t[\vec{k},s]}{\Delta t} \right|^2 \\
&+ \frac{1}{\hbar^2} \sum_{\vec{k}\in\mathbb{A}^s_{t+\Delta t}} \sum_{m:\vec{k}+\vec{e}_m\in\mathbb{A}^b_{t+\Delta t}} \left| \gamma_m(k_m+1)\hat{L}_m[s,s]\Psi_t[\vec{k},s] \right|^2 \\
&+ \frac{1}{\hbar^2} \sum_{\vec{k}\in\mathbb{A}^s_{t+\Delta t}} \sum_{m:\vec{k}+\vec{e}_m\in\mathbb{A}_{t+\Delta t}} \sum_{d\in\mathbb{S}^d_t\setminus\{s\}} \left| \gamma_m(k_m+1)\hat{L}_m[d,s]\Psi_t[\vec{k},s] \right|^2 \\
&+ \frac{1}{\hbar^2} \sum_{\vec{k}\in\mathbb{A}^s_{t+\Delta t}} \sum_{m:\vec{k}-\vec{e}_m\in\mathbb{A}^b_{t+\Delta t}} \left| \frac{g_m}{\gamma_m}(\hat{L}_m[s,s] - \langle\hat{L}_m\rangle_t\,\delta_{s,s})\Psi_t[\vec{k},s] \right|^2 \\
&+ \frac{1}{\hbar^2} \sum_{\vec{k}\in\mathbb{A}^s_{t+\Delta t}} \sum_{m:\vec{k}-\vec{e}_m\in\mathbb{A}_{t+\Delta t}} \sum_{d\in\mathbb{S}^d_t\setminus\{s\}} \left| \frac{g_m}{\gamma_m}(\hat{L}_m[d,s] - \langle\hat{L}_m\rangle_t\,\delta_{d,s})\Psi_t[\vec{k},s] \right|^2 \\
&+ \frac{1}{\hbar^2} \sum_{\vec{k}\in\mathbb{A}^s_{t+\Delta t}} \sum_{s'\in\mathbb{S}\setminus\{s\}} \left| (-i\hat{H}_S + \hat{Z}_t + \hat{T}^{(\vec{k})})[s',s]\Psi_t[\vec{k},s] \right|^2
\end{aligned}
\tag{S45}
$$

where we note that the numerical construction of $(\mathscr{L}_{\mathbb{A}^s_{t+\Delta t}\otimes\mathbb{S}_t}|\Psi_t\rangle)$ is performed as an additional derivative evaluation using the HOPS equation expressed in the reduced basis $\mathbb{A}^s_{t+\Delta t}\otimes\mathbb{S}_t$ with a HOPS wave function $|\Psi_t\rangle$ that has been updated to account for the reduced basis such that

$$
(\mathscr{L}_{\mathbb{A}^s_{t+\Delta t}\otimes\mathbb{S}_t}\Psi_t)[\vec{k},s] = \begin{cases} \frac{d}{dt}\Psi_t[\vec{k},s] \text{ if } \vec{k}\in\mathbb{A}^s_{t+\Delta t} \\ 0 \text{ otherwise.} \end{cases}
\tag{S46}
$$

#### *1. Stable State Basis*

Starting from Eq. (S45), we explicitly calculate the error contributions associated with excluding $|s\rangle \in \mathbb{S}_t$ from the basis $\mathbb{S}_{t+\Delta t}$ as described below. The two components of the flux-in error calculation

$$
E^2_{\mathbb{S}^s_t,\mathrm{in}}[\vec{k},s] = \left| \frac{d\Psi_t[\vec{k},s]}{dt} + \frac{\Psi_t[\vec{k},s]}{\Delta t} \right|^2
\tag{S47}
$$

are calculated together since they are able to cancel.

The diagonal portions (associated with diagonal elements of $\hat{L}_n$ in the Hilbert space of $\hat{H}_S$) of the flux-up

$$
\begin{aligned}
\hbar^2 E^2_{\mathbb{S}^s_t,\mathrm{up,diag}}[\vec{k},s] &= \sum_m \delta_{\vec{k}+\vec{e}_m\in\mathbb{A}^b_{t+\Delta t}} \left| (k_m+1)\gamma_m\hat{L}_m[s,s]\Psi_t[\vec{k},s] \right|^2 \\
&= \left|\Psi_t[\vec{k},s]\right|^2 \sum_m F_{\mathbb{S}^s_t,\mathrm{up,diag}}[\vec{k},m] \left| (k_m+1)\gamma_m\hat{L}_m[s,s] \right|^2 \\
&= \left|\Psi_t[\vec{k},s]\right|^2 \sum_m F_{\mathbb{S}^s_t,\mathrm{up,diag}}[\vec{k},m] \left| (k_m+1)\gamma_m M^{diag}[m,s] \right|^2
\end{aligned}
\tag{S48}
$$

and flux-down

$$
\begin{aligned}
\hbar^2 E^2_{\mathbb{S}^s_t,\mathrm{down,diag}}[\vec{k},s] &= \sum_m \delta_{\vec{k}-\vec{e}_m\in\mathbb{A}^b_{t+\Delta t}} \left| \frac{g_m}{\gamma_m}(\hat{L}_m[s,s] - \langle\hat{L}_m\rangle_t\,\delta_{s,s})\Psi_t[\vec{k},s] \right|^2 \\
&= \left|\Psi_t[\vec{k},s]\right|^2 \sum_m F_{\mathbb{S}^s_t,\mathrm{down,diag}}[\vec{k},m] \left| \frac{g_m}{\gamma_m}(\hat{L}_m[s,s] - \langle\hat{L}_m\rangle_t) \right|^2 \\
&= \left|\Psi_t[\vec{k},s]\right|^2 \sum_m F_{\mathbb{S}^s_t,\mathrm{down,diag}}[\vec{k},m] \left| \frac{g_m}{\gamma_m}\left(M^{diag} - X\right)[m,s] \right|^2
\end{aligned}
\tag{S49}
$$

error calculations are simplified by introducing the filters $F_{\mathbb{S}_t^s,\text{up,diag}}[\vec{k},m] = \delta_{\vec{k}+\vec{e}_m \in \mathbb{A}^b_{t+\Delta t}}$ and $F_{\mathbb{S}_t^s,\text{down,diag}}[\vec{k},m] = \delta_{\vec{k}-\vec{e}_m \in \mathbb{A}^b_{t+\Delta t}}$.

Conversely, the off-diagonal portions of the same flux-up

$$\begin{aligned}
\hbar^2 E^2_{\mathbb{S}_t^s,\text{up,off}}[\vec{k},s] &= \sum_m \delta_{\vec{k}+\vec{e}_m \in \mathbb{A}_{t+\Delta t}} \sum_{d \neq s \in \mathbb{S}_t^d} \left| (k_m+1)\gamma_m \hat{L}_m[d,s] \Psi_t[\vec{k},s] \right|^2 \\
&= \left|\Psi_t[\vec{k},s]\right|^2 \sum_m F_{\mathbb{S}_t^s,\text{up,off}}[\vec{k},m] \left|(k_m+1)\gamma_m\right|^2 \sum_{d \in \mathbb{S}_t^d \setminus \{s\}} \left|\hat{L}_m[d,s]\right|^2 \\
&= \left|\Psi_t[\vec{k},s]\right|^2 \sum_m F_{\mathbb{S}_t^s,\text{up,off}}[\vec{k},m] \left|(k_m+1)\gamma_m\right|^2 \left( \sum_{d \in \mathbb{S}_t^d} \left| M_d^{off} \right|^2 \right)[m,s]
\end{aligned} \tag{S50}$$

and flux-down

$$\begin{aligned}
\hbar^2 E^2_{\mathbb{S}_t^s,\text{down,off}}[\vec{k},s] &= \sum_m \delta_{\vec{k}-\vec{e}_m \in \mathbb{A}_{t+\Delta t}} \sum_{d \neq s \in \mathbb{S}_t^d} \left| \frac{g_m}{\gamma_m} (\hat{L}_m[d,s] - \langle \hat{L}_m \rangle_t \, \delta_{d,s}) \Psi_t[\vec{k},s] \right|^2 \\
&= \left|\Psi_t[\vec{k},s]\right|^2 \sum_m F_{\mathbb{S}_t^s,\text{down,off}}[\vec{k},m] \left|\frac{g_m}{\gamma_m}\right|^2 \sum_{d \in \mathbb{S}_t^d \setminus \{s\}} \left|\hat{L}_m[d,s]\right|^2 \\
&= \left|\Psi_t[\vec{k},s]\right|^2 \sum_m F_{\mathbb{S}_t^s,\text{down,off}}[\vec{k},m] \left|\frac{g_m}{\gamma_m}\right|^2 \left( \sum_{d \in \mathbb{S}_t^d} \left| M_d^{off} \right|^2 \right)[m,s]
\end{aligned} \tag{S51}$$

error calculations are simplified by introducing the filters $F_{\mathbb{S}_t^s,\text{up,off}}[\vec{k},m] = \delta_{\vec{k}+\vec{e}_m \in \mathbb{A}_{t+\Delta t}}$ and $F_{\mathbb{S}_t^s,\text{down,off}}[\vec{k},m] = \delta_{\vec{k}-\vec{e}_m \in \mathbb{A}_{t+\Delta t}}$.

The squared state-flux error is given by

$$\hbar^2 E^2_{\mathbb{S}_t^s,\text{state}}[s] = \sum_{\vec{k} \in \mathbb{A}^s_{t+\Delta t}} \sum_{s' \in \mathbb{S} \setminus \{s\}} \left| (-i\hat{H}_S + \hat{Z}_t + \hat{T}^{(\vec{k})})[s',s] \Psi_t[\vec{k},s] \right|^2. \tag{S52}$$

The total squared derivative error (Eq. (S45)) is thus

$$\begin{aligned}
E^2_{\mathbb{S}_t^s}[s] = &\sum_{\vec{k} \in \mathbb{A}^s_{t+\Delta t}} E^2_{\mathbb{S}_t^s,\text{in}}[\vec{k},s] \\
&+ \sum_{\vec{k} \in \mathbb{A}^s_{t+\Delta t}} \left( E^2_{\mathbb{S}_t^s,\text{up,diag}} + E^2_{\mathbb{S}_t^s,\text{up,off}} \right)[\vec{k},s] \\
&+ \sum_{\vec{k} \in \mathbb{A}^s_{t+\Delta t}} \left( E^2_{\mathbb{S}_t^s,\text{down,diag}} + E^2_{\mathbb{S}_t^s,\text{down,off}} \right)[\vec{k},s] \\
&+ E^2_{\mathbb{S}_t^s,\text{state}}[s].
\end{aligned} \tag{S53}$$

### 2. Boundary State Basis

Starting from Eq. (S45), we note that the derivative error associated with excluding a state $|s_b\rangle \in \mathbb{S} \setminus \mathbb{S}_t$ from the basis can stem only from the fluxes that change state index: that is, state flux and the off-diagonal portions of flux up and down. Because population has been deleted from terms excluded during construction of the stable state basis, we introduce $\mathbb{S}^s_{t+\Delta t}$, the stable state basis preserved from $\mathbb{S}_t$. The squared state-flux error derivative error is given by

$$\begin{aligned}
E^2_{\mathbb{S}_t^b,\text{state}}[s_b] &= \sum_{\vec{k} \in \mathbb{A}^s_{t+\Delta t}} \left| \sum_{s \in \mathbb{S}^s_{t+\Delta t}} \mathscr{L}[\vec{k},s_b,\vec{k},s] \Psi_t[\vec{k},s] \right|^2 \\
&= \frac{1}{\hbar^2} \sum_{\vec{k} \in \mathbb{A}^s_{t+\Delta t}} \left| \sum_{s \in \mathbb{S}^s_{t+\Delta t}} (-i\hat{H}_S + \hat{Z}_t + \hat{T}^{(\vec{k})})[s_b,s] \Psi_t[\vec{k},s] \right|^2
\end{aligned} \tag{S54}$$

where we have simplified the outer sum because boundary auxiliary vectors $|\vec{k}_b\rangle \in \mathbb{A}^b_{t+\Delta t}$ are unpopulated.

The flux-up and flux-down terms associated with populated states must be re-calculated to account for the states removed from the basis during the construction of $\mathbb{S}_t$. However, since we only consider fluxes going to states not in the current basis, only the off-diagonal portion of those fluxes (that is, the portion stemming from off-diagonal entries of the $\hat{L}_n$ in the Hilbert space of $\hat{H}_S$) must be considered.

We find an upper bound on the flux-up

$$\begin{aligned}\hbar^2 E^2_{\mathbb{S}^b_t,\mathrm{up,off}}[s_b] &= \sum_{\vec{k}\in\mathbb{A}^s_{t+\Delta t}} \hbar^2 E^2_{\mathbb{S}^b_t,\mathrm{up,off}}[\vec{k},s_b] \\ &= \sum_{\vec{k}\in\mathbb{A}^s_{t+\Delta t}} \sum_m \delta_{\vec{k}+\vec{e}_m\in\mathbb{A}_{t+\Delta t}} \left| \sum_{s\in\mathbb{S}^s_{t+\Delta t}} (k_m+1)\gamma_m \hat{L}_m[s_b,s]\Psi_t[\vec{k},s]\right|^2 \\ &\leq \sum_{\vec{k}\in\mathbb{A}^s_{t+\Delta t}} \sum_{s\in\mathbb{S}^s_{t+\Delta t}} \left|\Psi_t[\vec{k},s]\right|^2 \sum_m F_{\mathbb{S}^s_t,\mathrm{up,off}}[\vec{k},m] \left|(k_m+1)\gamma_m \hat{L}_m[s_b,s]\right|^2 \\ &\leq \sum_{\vec{k}\in\mathbb{A}^s_{t+\Delta t}} \sum_{s\in\mathbb{S}^s_{t+\Delta t}} \left|\Psi_t[\vec{k},s]\right|^2 \sum_m F_{\mathbb{S}^s_t,\mathrm{up,off}}[\vec{k},m] \left|(k_m+1)\gamma_m M^{off}_{s_b}[m,s]\right|^2\end{aligned} \tag{S55}$$

and flux-down

$$\begin{aligned}\hbar^2 E^2_{\mathbb{S}^b_t,\mathrm{down,off}}[s_b] &= \sum_{\vec{k}\in\mathbb{A}^s_{t+\Delta t}} \hbar^2 E^2_{\mathbb{S}^s_t,\mathrm{down,off}}[\vec{k},s_b] \\ &= \sum_{\vec{k}\in\mathbb{A}^s_{t+\Delta t}} \sum_m \delta_{\vec{k}-\vec{e}_m\in\mathbb{A}_{t+\Delta t}} \left| \sum_{s\in\mathbb{S}^s_{t+\Delta t}} \frac{g_m}{\gamma_m}(\hat{L}_m[s_b,s]-\langle \hat{L}_m\rangle_t \,\delta_{s_b,s})\Psi_t[\vec{k},s]\right|^2 \\ &\leq \sum_{\vec{k}\in\mathbb{A}^s_{t+\Delta t}} \sum_{s\in\mathbb{S}^s_{t+\Delta t}} \left|\Psi_t[\vec{k},s]\right|^2 \sum_m F_{\mathbb{S}^s_t,\mathrm{down,off}}[\vec{k},m] \left|\frac{g_m}{\gamma_m}\hat{L}_m[s_b,s]\right|^2 \\ &\leq \sum_{\vec{k}\in\mathbb{A}^s_{t+\Delta t}} \sum_{s\in\mathbb{S}^s_{t+\Delta t}} \left|\Psi_t[\vec{k},s]\right|^2 \sum_m F_{\mathbb{S}^s_t,\mathrm{down,off}}[\vec{k},m] \left|\frac{g_m}{\gamma_m} M^{off}_{s_b}[m,s]\right|^2\end{aligned} \tag{S56}$$

error calculations, where we re-use the filters from the stable basis. The upper bound imposed by summing over modes $m$ prior to states $s$ is purely for the sake of allowing the use of matrix multiplication in the code implementation, accelerating calculations.

The total squared derivative error (Eq. (S45)) is given by

$$\begin{aligned}E^2_{\mathbb{S}^b_t}[s_b] =& E^2_{\mathbb{S}^b_t,\mathrm{state}}[s_b] \\ &+E^2_{\mathbb{S}^b_t,\mathrm{up,off}}[s_b] \\ &+E^2_{\mathbb{S}^b_t,\mathrm{down,off}}[s_b].\end{aligned} \tag{S57}$$

## S3. DRUDE-LORENTZ SPECTRAL DENSITY

In all calculations presented here, we describe each independent environment ($n$) with an overdamped Drude-Lorentz spectral density

$$J_n(\omega) = 2\lambda_n\gamma_n \frac{\omega}{\omega^2+\gamma_n^2} \tag{S58}$$

where $\lambda_n$ is the reorganization energy and $\gamma_n$ is the reorganization timescale of the $n^{\mathrm{th}}$ environment. The associated exponential decomposition of the correlation function at temperature $T$ is given by a high-temperature mode, with magnitude $g_{\gamma_n}$ and decay frequency $\gamma_n$, and $k_{\mathrm{Mats}}$ Matsubara modes, with magnitudes $g_{\nu_n}$ and decay frequencies $\gamma_{\nu_n}$:

$$C_n(t) = g_{\gamma_n} e^{-\gamma_n t/\hbar} + \sum_{\nu=1}^{k_{\mathrm{Mats}}} g_{\nu_n} e^{-\gamma_{\nu_n} t/\hbar} \tag{S59}$$

where

$$g_{\gamma_n} = 2\lambda_n\beta^{-1}\left(1+\sum_{j_n=1}^{k_{\mathrm{Mats}}}\frac{\gamma_n^2}{\gamma_n^2-\gamma_{j_n}^2}\right) - i\lambda_n\gamma_n \tag{S60}$$

and

$$g_{\nu_n} = \frac{2i}{\beta} J_n(i\gamma_{\nu_n}), \quad \gamma_{\nu_n} = \frac{2\pi\nu}{\beta} \tag{S61}$$

where $\beta = \frac{1}{k_B T}$.

## S4. SIZE-INVARIANCE IN VARIOUS MODELS

MesoHOPS v1.6, based on the new adaptive algorithm described above, shows $\mathcal{O}(1)$ scaling with system-bath coupling operators that have either diagonal or off-diagonal components. Fig. S1 shows CPU time vs number of molecules ($N$) for linear chains: (a) one excitation with

$$\hat{H}_S = \sum_{n=1}^{N} V \left|n\right\rangle \left\langle n+1\right| + h.c. \tag{S62}$$

and Holstein vibrations ($L_n = \left|n\right\rangle \left\langle n\right|$), (b) two excitations with

$$\hat{H}_S = \sum_{n=1}^{N} \sum_{m=1}^{n} V \Big( \left|n,m\right\rangle \left\langle n \pm 1, m\right| + \left|n,m\right\rangle \left\langle n, m \pm 1\right| \Big) + h.c. \tag{S63}$$

and Holstein vibrations ($L_n = 2\left|n,n\right\rangle \left\langle n,n\right| + \sum_{m \neq 0} \left|n,m\right\rangle \left\langle n,m\right|$), and (c) one excitation ($\hat{H}_S$ given by Eq. (S62)) and Peierls vibrations ($L_n = \left|n\right\rangle \left\langle n+1\right| + h.c.$).

In all cases, we note the onset of size-invariant scaling by $N = 30$, illustrating the power and flexibility of the updated adaptive algorithm. We attribute the greater CPU time to greater delocalization extents in the Peierls case, and to the fact that a pair of particles each physically delocalized over $r_P$ sites populates $r_P^2$ states in the 2-particle Holstein case.

All calculations reported in Fig. S1 use matched parameters, where each bath is characterized by a Drude-Lorentz spectral density with $\lambda_n = \gamma_n = V = 50$ cm$^{-1}$ and a temperature of 300 K. The initial system state is $\left|1\right\rangle$ for the one-particle calculations and $\left|0,N\right\rangle$ for the two-particle calculations. All calculations are run out to 2 ps.

Finally, we note that the onset of size-invariance requires a system with a handful of physical properties:

1. Sufficiently strong system-bath interactions to localize excitations: materials in which transport is fully band-like will not exhibit size-invariance.

2. Local couplings between excited states, such that there is some cutoff distance beyond which excited states do not interact: otherwise, increasing the extent of a system will always result in a given excited state being coupled to a greater number of excited states, increasing delocalization extents and the size of the destination state basis $\mathbb{S}_t^d$.

3. Finite reorganization time of the bath: otherwise, auxiliary wave functions associated with excited states populated at any given point in time will remain populated, and the adaptive algorithm will not truncate them from the basis.

The first condition is generally true for molecular materials, and the latter two hold for any realistic material: thus, we expect that simulations of any relevant system will eventually reach size-invariance. Nonetheless, in systems with sufficiently weak system-bath interactions, long-range couplings, and long reorganization times, reaching the onset of size-invariance may prove inconvenient.

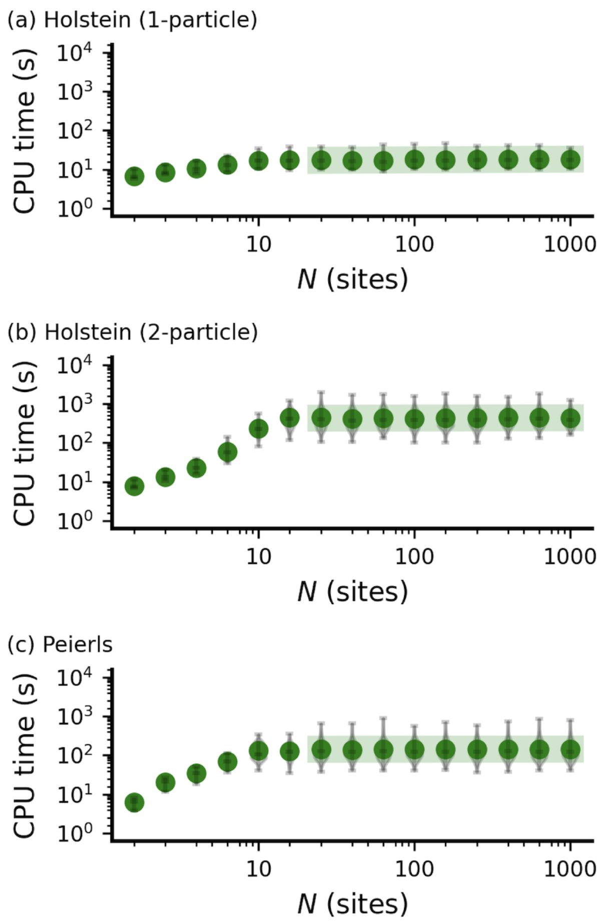


FIG. S1. Size-invariance in various models. All CPU times were measured by running each trajectory on a single thread of an AMD EPYC 9534 64-Core Processor.

## S5. THE PDI HAMILTONIAN

We consider a model that consists of a linear chain of $N$ identical N,N'-Bis(2-phenylethyl)-3,4,9,10-perylenedi-carboximide (EP-PDI) molecules. Each individual molecule ($n$) may host a singlet exciton state $|e_n\rangle$. Pairs of adjacent molecules $(n, n+1)$ may host the charge transfer (CT) states $|A_nC_{n+1}\rangle$ and $|C_nA_{n+1}\rangle$, where $A$ denotes the anionic molecule and $C$ denotes the cationic molecule. Each adjacent pair may also host the triplet-pair (TT) state $|T_nT_{n+1}\rangle$ with identical triplet excitations on molecules $n$ and $n+1$.

Following Ref. 8, $\hat{H}_S$ is given by the sum of several parts: first, the vertical excitation energies of each state:

$$\sum_{n=1}^{N} E_S |e_n\rangle\langle e_n| + \sum_{n=1}^{N-1} E_{TT} |T_nT_{n+1}\rangle\langle T_nT_{n+1}| + \sum_{n=1}^{N-1} E_{CT} \left(|A_nC_{n+1}\rangle\langle A_nC_{n+1}| + |C_nA_{n+1}\rangle\langle C_nA_{n+1}|\right) \tag{S64}$$

Second, direct 2-electron couplings ($V_{2e}$) between each TT state occupying $(n,\ n+1)$ and the singlet states on sites $n$ and $n+1$:

$$\sum_{n=1}^{N-1} V_{2e}\left(|e_n\rangle\langle T_nT_{n+1}| + |e_{n+1}\rangle\langle T_nT_{n+1}|\right) + h.c. \tag{S65}$$

Third, 1-electron couplings between the CT states occupying $(n,\ n+1)$ and the singlet states on sites $n$ and $n+1$. Because we have defined the diabatic electronic states based on the highest occupied molecular orbital (HOMO) and lowest unoccupied molecular orbital

(LUMO) of each molecule, the couplings between these states are either HOMO-HOMO ($V_{HH}$) or LUMO-LUMO ($V_{LL}$) couplings:[8,9]

$$\begin{aligned}&\sum_{n=1}^{N-1}(V_{LL}\left|e_n\right\rangle\left\langle C_nA_{n+1}\right| - V_{HH}\left|e_{n+1}\right\rangle\left\langle C_nA_{n+1}\right|) + h.c.\\ &+\sum_{n=1}^{N-1}(V_{LL}\left|e_{n+1}\right\rangle\left\langle A_nC_{n+1}\right| - V_{HH}\left|e_n\right\rangle\left\langle A_nC_{n+1}\right|) + h.c.\end{aligned} \tag{S66}$$

Finally, 1-electron couplings between the CT states and TT states occupying the same pair of molecules ($n$, $n+1$). These couplings are either HOMO-LUMO ($V_{HL}$) or LUMO-HOMO ($V_{LH}$) couplings:

$$\begin{aligned}&\sum_{n=1}^{N-1}\sqrt{\frac{3}{2}}V_{HL}(\left|T_nT_{n+1}\right\rangle\left\langle C_nA_{n+1}\right|) + h.c.\\ &+\sum_{n=1}^{N-1}\sqrt{\frac{3}{2}}V_{LH}(\left|T_nT_{n+1}\right\rangle\left\langle A_nC_{n+1}\right|) + h.c.\end{aligned} \tag{S67}$$

To explore the role of vibrations in the mechanism of SF, we consider three vibrational models. In all models, each state $|s\rangle$ is coupled to an identical independent Holstein bath with system-bath coupling operator

$$\hat{L}_s^H = |s\rangle\langle s| \tag{S68}$$

and a Drude-Lorentz spectral density parametrized by $\lambda_H$ and $\gamma_H$. The three models enumerated below differ in their treatment of Peierls vibrations:

1. **Holstein Model**: This model ignores the possibility of Peierls vibrations.

2. **Direct Coupling Peierls Model**: This model is adapted from previous simulations of an EP-PDI dimer, which found that fluctations in the direct couplings between the singlets and TT states, described by system-bath coupling operators

$$\hat{L}_{n^+}^{2e} = \left|e_n\right\rangle\left\langle T_nT_{n+1}\right| + h.c.,\ \hat{L}_{n^-}^{2e} = \left|e_n\right\rangle\left\langle T_{n-1}T_n\right| + h.c. \tag{S69}$$

   and parametrized by a Drude-Lorentz spectral density with $\lambda_P^{2e}$ and $\gamma_P^{2e}$, increase the fission rate by orders of magnitude.[10]

3. **CT-Mediated Coupling Peierls Model**: This model is based on simulations of a pentacene dimer, which found that the role of Peierls vibrations lies in breaking the anti-symmetric effects that inhibit CT-mediated singlet fission.[11] The most direct way to achieve this is by modulating the couplings between CT and TT states with system-bath coupling operators

$$\hat{L}_n^{HL} = \left|T_nT_{n+1}\right\rangle\left\langle C_nA_{n+1}\right| + h.c. \tag{S70}$$

   and

$$\hat{L}_n^{LH} = \left|T_nT_{n+1}\right\rangle\left\langle A_nC_{n+1}\right| + h.c. \tag{S71}$$

   We assume these Peierls vibrations are described by identical Drude-Lorentz spectral densities given by $\lambda_P^{HL} = \lambda_P^{LH}$ and $\gamma_P^{HL} = \gamma_P^{LH}$.

The Hamiltonian parameters for all models are given in Table S2, and all parameters are adapted from Ref. 10, except for $\lambda_P^{HL}$, which is obtained by rescaling $\lambda_P^{2e}$ to the ratio $|V_{HL}/V_{2e}|$, yielding baths similar to those in a previous parametrization of Peierls vibrations in pentacene dimers.[11]

In periodic systems, we introduce additional states $|T_NT_1\rangle$, $|C_NA_1\rangle$, and $|A_NC_1\rangle$, and couplings between states are defined in a periodic fashion such that $N+1$ is interchangeable with 1. The periodic dimer in Fig. 5 of the main text, which effectively double-counts the CT and TT states, is a fictitious system that illustrates limiting periodic behavior.

The timescale of singlet diffusion is difficult to calculate due to rapid singlet fission. To circumvent this complexity, we isolate singlet diffusion in Fig. 5.d of the main text (bright blue lines) by removing all triplet pair states (including associated electronic couplings and vibrational baths) from the Hamiltonian.

All calculations were run at 300 K, with the initial state $|\psi_0^{(\vec{0})}\rangle = \sum_{n=1}^{N}\frac{1}{\sqrt{N}}|e_n\rangle$, except in

- Fig 4.b (blue) of the main text, where the one-singlet model has the initial state $|e_1\rangle$.
- Fig 4.c (cyan) of the main text, where we test initial state $\frac{1}{\sqrt{2}}\Big(|e_1\rangle - |e_2\rangle\Big)$.
- Fig 5.d-e of the main text, where the initial state is $|e_1\rangle$ for the singlet MSD (light blue) and $|T_1T_2\rangle$ for the triplet MSD (black, dark blue).
- Fig 5.f of the main text, where the initial state of each trajectory is $|e_n\rangle$, where $n$ is a randomly-selected site (using a localized initial state allows for a *ceteris paribus* analysis of adHOPS scaling with respect to system size).

| Parameter | Value (cm$^{-1}$) |
|---|---|
| $E_S$ | 17500 |
| $E_{TT}$ | 15300 |
| $E_{CT}$ | 25100 |
| $V_{2e}$ | -3.39 |
| $V_{LL}$ | 1170 |
| $V_{HH}$ | -968 |
| $V_{HL}$ | -968 |
| $V_{LH}$ | 968 |
| $\lambda_H$ | 621 |
| $\gamma_H$ | 1210 |
| $\lambda_P^{2e}$ | 0.726 |
| $\gamma_P^{2e}$ | 161 |
| $\lambda_P^{HL} = \lambda_P^{LH}$ | 217 |
| $\gamma_P^{HL} = \gamma_P^{LH}$ | 161 |

TABLE S2. Parametrizing the PDI Hamiltonian (values converted from meV, reported to 3 significant figures).

## A. MSD Calculations

We find mean-squared diffusion (MSD) of the singlet and triplet pair states by taking the expectation value of a mean-squared diffusion operator for each of those states

$$\hat{D}_S = \sum_{n=1}^{N} (Ln)^2 |e_n\rangle\langle e_n|; \;\; \hat{D}_{TT} = \sum_{n=1}^{N-1} (Ln)^2 |T_n T_{n+1}\rangle\langle T_n T_{n+1}| \tag{S72}$$

where $L$ is the distance between EP-PDI molecules (taken to be 3.28 Å, following Ref. 12). The expectation values of the diffusion operators are taken with the physical wave function normalized to the total population of the associated state using the singlet and triplet pair projection operators,

$$\hat{P}_S = \sum_{n=1}^{N} |e_n\rangle\langle e_n|; \;\; \hat{P}_{TT} = \sum_{n=1}^{N-1} |T_n T_{n+1}\rangle\langle T_n T_{n+1}| \tag{S73}$$

such that

$$\text{MSD}(t) = \frac{\langle \hat{D}_S \rangle_t}{\langle \hat{P}_S \rangle_t}; \;\; \text{MSD}(t) = \frac{\langle \hat{D}_{TT} \rangle_t}{\langle \hat{P}_{TT} \rangle_t} \tag{S74}$$

for the singlet and for the triplet excited states, respectively.

## S6. EFFECTIVE COUPLINGS IN THE PDI MODEL

PDI exhibits excitation transfer from singlet states to TT states via the CT-mediated pathway, as well as between adjacent singlet states. However, neither of these pathways are represented directly by a coupling term in the Hamiltonian $\hat{H}_S$. Instead, we estimate them using a variation on perturbation theory to expand the states of interest in the CT states to first order, following similar logic to that of Eqs. 9-10 of Ref. 13. The effective CT-mediated coupling between states $|s\rangle$ and $|s'\rangle$, $\langle s|\hat{V}_{\text{eff}}|s'\rangle$ is

$$\langle s^{(1)}|\hat{H}_S^{off}|s'^{(1)}\rangle - \langle s|\hat{H}_S^{off}|s'\rangle \tag{S75}$$

where $\hat{H}_S^{off}$ is the off-diagonal portion of the time-dependent augmented system Hamiltonian corresponding to couplings between electronic states, and the first-order perturbation theory expansion of $|s\rangle$ through the CT states is given

$$|s^{(1)}\rangle = |s\rangle + \sum_{CT} \frac{\langle CT|\hat{H}_S|s'\rangle\,|CT\rangle}{\langle s|\hat{H}_S|s\rangle - \langle CT|\hat{H}_S|CT\rangle}\Big) \tag{S76}$$

where $CT$ is an index over all CT states and $\hat{H}_S$ is the total time-dependent augmented system Hamiltonian. Thus,

$$\langle s|\hat{V}_{\text{eff}}|s'\rangle = \Big(\langle s| + \sum_{CT} \frac{\langle s|\hat{H}_S|CT\rangle\,\langle CT|}{\langle s|\hat{H}_S|s\rangle - \langle CT|\hat{H}_S|CT\rangle}\Big)\hat{H}_S^{off}\Big(|s'\rangle + \sum_{CT} \frac{\langle CT|\hat{H}_S|s'\rangle\,|CT\rangle}{\langle s'|\hat{H}_S|s'\rangle - \langle CT|\hat{H}_S|CT\rangle}\Big) - \langle s|\hat{H}_S|s'\rangle \tag{S77}$$

### A. J-Aggregate-Like Singlet Nearest-Neighbor Coupling

To obtain the effective coupling between nearest-neighbor singlets $|e_n\rangle$ and $|e_{n+1}\rangle$, we begin by expanding

$$\langle e_n^{(1)}| = \langle e_n| + \frac{\langle e_n|\hat{H}_S|A_nC_{n+1}\rangle\,\langle A_nC_{n+1}|}{\langle e_n|\hat{H}_S|e_n\rangle - \langle A_nC_{n+1}|\hat{H}_S|A_nC_{n+1}\rangle} + \frac{\langle e_n|\hat{H}_S|C_nA_{n+1}\rangle\,\langle C_nA_{n+1}|}{\langle e_n|\hat{H}_S|e_n\rangle - \langle C_nA_{n+1}|\hat{H}_S|C_nA_{n+1}\rangle} + a\,\langle A_{n-1}C_n| + b\,\langle C_{n-1}A_n|. \tag{S78}$$

We will not expand $a$ and $b$, as they will not impact the effective coupling. Similarly, we expand

$$|e_{n+1}^{(1)}\rangle = |e_{n+1}\rangle + \frac{\langle e_{n+1}|\hat{H}_S|A_nC_{n+1}\rangle\,|A_nC_{n+1}\rangle}{\langle e_{n+1}|\hat{H}_S|e_{n+1}\rangle - \langle A_nC_{n+1}|\hat{H}_S|A_nC_{n+1}\rangle} + \frac{\langle e_{n+1}|\hat{H}_S|C_nA_{n+1}\rangle\,|C_nA_{n+1}\rangle}{\langle e_{n+1}|\hat{H}_S|e_{n+1}\rangle - \langle C_nA_{n+1}|\hat{H}_S|C_nA_{n+1}\rangle} + c\,|A_{n+1}C_{n+2}\rangle + d\,|C_{n+1}A_{n+2}\rangle. \tag{S79}$$

Because $\hat{H}_S^{off}$ has no diagonal components, $|e_{n+1}\rangle$ is not coupled to the CT states associated with the pair of molecules $(n-1, n)$, and $|e_n\rangle$ is not coupled to the CT states associated with the pair of molecules $(n+1, n+2)$:

$$\langle e_n|\hat{H}_S^{off}|A_{n+1}C_{n+2}\rangle = \langle e_n|\hat{H}_S^{off}|C_{n+1}A_{n+2}\rangle = \langle e_{n+1}|\hat{H}_S^{off}|A_{n-1}C_n\rangle = \langle e_{n+1}|\hat{H}_S^{off}|C_{n-1}A_n\rangle = \langle s|\hat{H}_S^{off}|s\rangle = 0. \tag{S80}$$

Finally, we also note there is no direct coupling in $\hat{H}_S^{off}$ between any two CT states, nor between any two singlet states.

Thus, to solve the effective CT-mediated coupling between neighboring singlet states

$$\langle e_n|\hat{V}_{NN}|e_{n+1}\rangle = \langle e_n^{(1)}|\hat{H}_S^{off}|e_{n+1}^{(1)}\rangle - \langle s|\hat{H}_S^{off}|s'\rangle \tag{S81}$$

we only need to consider the four terms where $\hat{H}_S^{off}$ couples a singlet and CT state:

$$\langle e_n|\hat{V}_{NN}|e_{n+1}\rangle = \frac{\langle e_n|\hat{H}_S|A_nC_{n+1}\rangle\,\langle A_nC_{n+1}|\hat{H}_S^{off}|e_{n+1}\rangle}{\langle e_n|\hat{H}_S|e_n\rangle - \langle A_nC_{n+1}|\hat{H}_S|A_nC_{n+1}\rangle} + \frac{\langle e_n|\hat{H}_S|C_nA_{n+1}\rangle\,\langle C_nA_{n+1}|\hat{H}_S^{off}|e_{n+1}\rangle}{\langle e_n|\hat{H}_S|e_n\rangle - \langle C_nA_{n+1}|\hat{H}_S|C_nA_{n+1}\rangle} \tag{S82}$$

$$+ \frac{\langle A_nC_{n+1}|\hat{H}_S|e_{n+1}\rangle\,\langle e_n|\hat{H}_S^{off}|A_nC_{n+1}\rangle}{\langle e_{n+1}|\hat{H}_S|e_{n+1}\rangle - \langle A_nC_{n+1}|\hat{H}_S|A_nC_{n+1}\rangle} + \frac{\langle C_nA_{n+1}|\hat{H}_S|e_{n+1}\rangle\,\langle e_n|\hat{H}_S^{off}|C_nA_{n+1}\rangle}{\langle e_{n+1}|\hat{H}_S|e_{n+1}\rangle - \langle C_nA_{n+1}|\hat{H}_S|C_nA_{n+1}\rangle}. \tag{S83}$$

If the noise and noise memory drift are both ignored, this is

$$\frac{4V_{HH}V_{LL}}{E_{CT} - E_S} = -621\ \text{cm}^{-1}. \tag{S84}$$

Naturally, $\langle e_{n+1}|\hat{V}_{NN}|e_n\rangle = \langle e_n|\hat{V}_{NN}|e_{n+1}\rangle^*$.

### B. Effective Coupling of the CT-Mediated Mechanism

To obtain the effective mediated coupling between states $|e_n\rangle$ and $|T_nT_{n+1}\rangle$, we expand $|e_n^{(1)}\rangle$ as above, and

$$|T_nT_{n+1}^{(1)}\rangle = |T_nT_{n+1}^{(1)}\rangle + \frac{\langle C_nA_{n+1}|\hat{H}_S|T_nT_{n+1}\rangle\,|C_nA_{n+1}\rangle}{\langle T_nT_{n+1}|\hat{H}_S|T_nT_{n+1}\rangle - \langle C_nA_{n+1}|\hat{H}_S|C_nA_{n+1}\rangle} + \frac{\langle A_nC_{n+1}|\hat{H}_S|T_nT_{n+1}\rangle\,|A_nC_{n+1}\rangle}{\langle T_nT_{n+1}|\hat{H}_S|T_nT_{n+1}\rangle - \langle A_nC_{n+1}|\hat{H}_S|A_nC_{n+1}\rangle}. \tag{S85}$$

is similarly given by first-order perturbation theory through the CT states. Plugging in

$$\langle e_n|\,\hat{V}_{\text{med}}\,|T_nT_{n+1}\rangle = \langle n_S^{(1)}|\hat{H}_S^{off}|TT_nT_{n+1}^{(1)}\rangle - \langle n_S|\hat{H}_S^{off}|TT_nT_{n+1}\rangle \tag{S86}$$

the direct coupling between the singlet and TT state vanishes, and because $\hat{H}_S^{off}$ does not directly couple the CT states to each other, we are left once again with only four terms:

$$\langle e_n|\,\hat{V}_{\text{med}}\,|T_nT_{n+1}\rangle = \frac{\langle e_n|\hat{H}_S|C_nA_{n+1}\rangle\,\langle C_nA_{n+1}|\hat{H}_S^{off}|T_nT_{n+1}\rangle}{\langle e_n|\hat{H}_S|e_n\rangle - \langle C_nA_{n+1}|\hat{H}_S|C_nA_{n+1}\rangle} + \frac{\langle e_n|\hat{H}_S|A_nC_{n+1}\rangle\,\langle A_nC_{n+1}|\hat{H}_S^{off}|T_nT_{n+1}\rangle}{\langle e_n|\hat{H}_S|e_n\rangle - \langle A_nC_{n+1}|\hat{H}_S|A_nC_{n+1}\rangle} \tag{S87}$$

$$+ \frac{\langle C_nA_{n+1}|\hat{H}_S|T_nT_{n+1}\rangle\,\langle e_n|\hat{H}_S^{off}|C_nA_{n+1}\rangle}{\langle T_nT_{n+1}|\hat{H}_S|T_nT_{n+1}\rangle - \langle C_nA_{n+1}|\hat{H}_S|C_nA_{n+1}\rangle} + \frac{\langle A_nC_{n+1}|\hat{H}_S|T_nT_{n+1}\rangle\,\langle e_n|\hat{H}_S^{off}|A_nC_{n+1}\rangle}{\langle T_nT_{n+1}|\hat{H}_S|T_nT_{n+1}\rangle - \langle A_nC_{n+1}|\hat{H}_S|A_nC_{n+1}\rangle}. \tag{S88}$$

Likewise, the effective coupling between $|e_{n+1}\rangle$ and $|T_nT_{n+1}\rangle$is

$$\langle e_n|\,\hat{V}_{\text{med}}\,|T_nT_{n+1}\rangle = \frac{\langle e_{n+1}|\hat{H}_S|C_nA_{n+1}\rangle\,\langle C_nA_{n+1}|\hat{H}_S^{off}|T_nT_{n+1}\rangle}{\langle e_{n+1}|\hat{H}_S|e_{n+1}\rangle - \langle C_nA_{n+1}|\hat{H}_S|C_nA_{n+1}\rangle} + \frac{\langle e_{n+1}|\hat{H}_S|A_nC_{n+1}\rangle\,\langle A_nC_{n+1}|\hat{H}_S^{off}|T_nT_{n+1}\rangle}{\langle e_{n+1}|\hat{H}_S|e_{n+1}\rangle - \langle A_nC_{n+1}|\hat{H}_S|A_nC_{n+1}\rangle} \tag{S89}$$

$$+ \frac{\langle C_nA_{n+1}|\hat{H}_S|T_nT_{n+1}\rangle\,\langle e_{n+1}|\hat{H}_S^{off}|C_nA_{n+1}\rangle}{\langle T_nT_{n+1}|\hat{H}_S|T_nT_{n+1}\rangle - \langle C_nA_{n+1}|\hat{H}_S|C_nA_{n+1}\rangle} + \frac{\langle A_nC_{n+1}|\hat{H}_S|T_nT_{n+1}\rangle\,\langle e_{n+1}|\hat{H}_S^{off}|A_nC_{n+1}\rangle}{\langle T_nT_{n+1}|\hat{H}_S|T_nT_{n+1}\rangle - \langle A_nC_{n+1}|\hat{H}_S|A_nC_{n+1}\rangle}. \tag{S90}$$

The magnitude of these effective couplings is approximately 48.4 $\text{cm}^{-1}$ in the absence of noise and noise memory drift. The anti-symmetry between $V_{HL}$ and $V_{LH}$, which stems from orbital geometry, is the limiting factor in the magnitude of the effective coupling and inhibits the CT-mediated mechanism.[11]

## S7. CONVERGENCE

### A. Calculation Parameters

Here, we describe in detail the parameters used to run adHOPS calculations.

#### 1. Hierarchy Depth $k_{max}$

We define a cutoff depth for the auxiliary wave functions, such that when $\|\vec{k}\|_1 > k_{\text{max}}$, HOPS sets the associated auxiliary wave function $|\psi_t^{(\vec{k})}\rangle = 0$. Increasing $k_{\text{max}}$ leads to more-converged calculations.

#### 2. Number of Matsubara Modes $k_{Mats}$

We decompose the Drude-Lorentz spectral densities used in our calculations into a sum of complex exponential modes: a single high-temperature mode and $k_{\text{Mats}}$ Matsubara modes. The explicit form of these modes is given in section S3. Increasing $k_{\text{Mats}}$ leads to more-converged calculations.

We denote Matsubara modes with the form $k_{\text{Mats}} = a/b$ to indicate that $a$ Matsubara modes were included in the decomposition, but the $b$ highest-frequency Matsubara modes were treated with a Markovian filter, which allows the first-order auxiliary wave function $|\psi_t^{(\vec{e}_v)}\rangle$ to be included in the hierarchy, but removes all other auxiliary wave functions $|\psi_t^{(\vec{k})}\rangle$ where $k_v > 0$.[5] Treating fewer Matsubara modes with a Markovian filter leads to more-converged calculations (that is, a higher value of $a$ and a lower value of $b$ indicate more-converged calculations).

In calculations run with multiple dissimilar baths requiring independent parametrization (i.e., both Holstein and Peierls vibrations), we use the form $k_{\text{Mats}} = a/b, c/d$, where $a/b$ refers to the Matsubara modes of the Holstein baths and $c/d$ to the Matsubara modes of the Peierls baths.

#### 3. Integration Time Step $dt$

We integrate the HOPS equation-of-motion with a fourth-order Runge-Kutta integrator over the time step $dt$. In principle, this time step may vary over the course of a calculation, but in our case it remains static. Decreasing $dt$ leads to more-converged calculations.

#### 4. Adaptive Error Bounds $\delta_A$ and $\delta_S$

The adaptive error bounds, as laid out above, act as phenomenological convergence parameters with monotonic behavior[1,5,14]. Decreasing $\delta_A$ and $\delta_S$ leads to more-converged calculations. When $\delta_A = \delta_S = 0$, adHOPS reverts to non-adaptive HOPS.

#### 5. Basis Update Time $u_t$

Calculating the adaptive error terms and updating the basis is the most time-consuming portion of most adHOPS calculations. The user may elect to update the adaptive bases only every $u_t$ (defined as an integer multiple of $dt$) to reduce the difficulty of simulation. Decreasing $u_t$ leads to more-converged calculations.

#### 6. Ensemble Size $N_{traj}$

In the HOPS formalism, calculated dynamics are given by an ensemble average over trajectories. The number of trajectories, $N_{\text{traj}}$, determines the quality of the statistical sampling. Following previous work[1,5,14], we use on the order of 1000 trajectories throughout our calculations presented here for the calculation of any dynamics. Increasing $N_{\text{traj}}$ leads to more-converged calculations.

#### 7. Discard Fraction ($f_{dis}$)

During the calculation of the boundary auxiliary basis (Section S2 A 2),the primary computational barrier is matching the flux terms to the associated boundary auxiliary wave functions. However, the majority of these terms are small enough that it is unlikely they will have an effect on the final result of basis construction. Thus, prior to matching error terms to boundary auxiliary terms $|\vec{k}_b\rangle \in \mathbb{A} \setminus \mathbb{A}_t$, the algorithm discards the maximum number of terms with errors that sum to less than $f_{\text{dis}}(\delta_A^2 - E_{\mathbb{A}_t^s}^2)$, where $f_{dis} \in [0,1]$. The remaining error terms are fed back into Eq. (S43), and the boundary auxiliary basis is constructed to satisfy error bound $(1 - f_{\text{dis}})(\delta_A^2 - E_{\mathbb{A}_t^s}^2)$. Thus, the error from the discarded terms is still taken into account. Note that $f_{\text{dis}}$ is not directly a convergence parameter: rather, it determines the convergence behavior of $\delta_A$. In all calculations shown, we set $f_{\text{dis}} = 0.01$.

#### 8. Early Time Basis Construction

Because the dynamics of a HOPS trajectory proceed rapidly at early time, it is necessary to aggressively grow the early-time basis to ensure accurate adHOPS calculations. To ensure a sufficiently large basis at early time, we iteratively call the adaptive basis algorithm at early time points, but remove no elements from the basis. The number of iterations done at each time point and the number of time points where the early time algorithm is used are user-defined variables. Following previous findings,[5] we use 2 inchworming iterations for the first 10 time points of each calculation.

#### 9. Effective Integration of the Noise

In all calculations shown in the main text, we used the effective integration of the noise laid out in Ref. 5, a method of smoothing the noise to capture ultrafast stochastic fluctuations, to increase the convenience of converging $dt$.

### B. Convergence Testing

To demonstrate the convergence of adHOPS calculations, we run multiple instances of the same calculations in ensembles of a given set of noise trajectories with less- and more-converged parameters. We measure convergence by taking the expectation value of some

observable at time $t$ as a function of the list of convergence parameters, $\mathbf{c}$:

$$\langle \hat{A} \rangle_t (\mathbf{c}) = \mathbb{E}_{\mathbf{z}}[\langle \psi_t^{(\vec{0})}(\mathbf{c})|\hat{A}|\psi_t^{(\vec{0})}(\mathbf{c})\rangle] \tag{S91}$$

where $\psi_t^{(\vec{0})}(\mathbf{c})$ is the system wave function of a trajectory run with convergence parameters $\mathbf{c}$ and $\hat{A}$ may be a scalar or vector observable. Comparing to an over-converged reference calculation with convergence parameters $\mathbf{c}'$ yields a measure of error that takes the form of a list over time

$$E_t(\mathbf{c}) = \| \langle \hat{A} \rangle_t (\mathbf{c}') - \langle \hat{A} \rangle_t (\mathbf{c}) \|_1 . \tag{S92}$$

The mean of $E_t(\mathbf{c})$ across time thus serves as a quantitative measure of convergence. The choice of observable should reflect the data being collected from a calculation. For the simple Peierls linear chain model, we analyzed the total population from a vectorized set of state projection operators

$$\hat{P}_{\text{tot}} = \sum_{s \in \mathbb{S}} |s\rangle \langle s| \vec{e}_s \tag{S93}$$

where $\{\vec{e}_i\}$ are mutually orthogonal unit vectors. For singlet fission calculations, we analyzed the sum population of all TT states, a scalar observable given by

$$\hat{P}_{\text{TT}} = \sum_{n=1}^{N-1} |T_n T_{n+1}\rangle \langle T_n T_{n+1}| . \tag{S94}$$

#### 1. Peierls Linear Chain Model

We found that, for converged calculations of the linear chains presented in Fig. 1 of the main text, $k_{\text{max}} = 15$, $dt = 4.0$ fs, $\delta_A = 0.001$, and $\delta_S = 0.001$. We determined these parameters by the satisfaction of a mean error less than 0.05 with $N_{\text{traj}} = 1000$ using the total population error (Eq. (S93)) with respect to a single reference ensemble with all-around tighter convergence parameters. We neglected Matsubara modes as a result of high temperature relative to the reorganization timescale.

#### 2. Singlet Fission in PDI

We found that, for converged calculations of the PDI dimers presented in Figs. 2-4 of the main text,

- $k_{\text{max}} = 3$, $k_{\text{Mats}} = 5/4$ (Holstein), $dt = 0.4$ fs for the model without Peierls vibrations.
- $k_{\text{max}} = 3$, $k_{\text{Mats}} = 5/4$ (Holstein), $k_{\text{Mats}} = 0/0$ (Peierls), $dt = 0.4$ fs for the model with Peierls vibrations modulating the direct singlet-TT coupling.
- $k_{\text{max}} = 3$, $k_{\text{Mats}} = 10/8$ (Holstein), $k_{\text{Mats}} = 0/0$ (Peierls), $dt = 0.2$ fs for the model with Peierls vibrations modulating the CT-TT couplings.

We determined these parameters by the satisfaction of a mean error less than 0.05 with $N_{\text{traj}} = 1000$ using the total population error TT population error (Eq. (S94)) with respect to a single reference ensemble with all-around tighter convergence parameters. We assumed that convergence parameters remained converged in the one-singlet model and when changing the initial system state.

We found that, for converged calculations of the linear chains with Peierls vibrations presented in Fig. 5 of the main text, $k_{\text{max}} = 3$, $k_{\text{Mats}} = 10/8$ (Holstein), $k_{\text{Mats}} = 0/0$ (Peierls), $dt = 0.2$ fs, $\delta_A = 0.01$, $\delta_S = 0.005$, and $u_t = 4.0$ fs. We determined these parameters by the satisfaction of a mean error of 0.02 in the linear chain tetramer model with $N_{\text{traj}} = 1000$ using the TT population error (Eq. (S94)) for $k_{\text{max}}$, $k_{\text{Mats}}$ (Peierls), $k_{\text{Mats}}$ (Holstein), $dt$, $\delta_A$, $\delta_S$, and $u_t$ separately. We assumed that convergence parameters remained converged in the periodic model and when changing the initial system state.

For converged calculations of linear chains without Peierls vibrations in Fig. 5 of the main text, $k_{\text{max}} = 3$, $k_{\text{Mats}} = 5/4$ (Holstein), $dt = 0.4$ fs, $\delta_A = 0.001$, $\delta_S = 0.001$, and $u_t = 4.0$ fs. We determined adaptive convergence parameters by satisfaction of a mean error of 0.02 in the linear chain model with $N_{\text{traj}} = 1000$ using the TT population error (Eq. (S94)): to determine $\delta_A$ and $u_t$, we compared a non-adaptive and adaptive calculation of a tetramer with $k_{\text{max}}$, $k_{\text{Mats}}$ (Peierls), $k_{\text{Mats}}$ (Holstein), and $dt$ based on the converged values in the dimer model. To determine $\delta_S$, we compared calculations of the decamer with all other parameters set to those converged for the tetramer against a reference $\delta_S = 0$.

The error calculations used to determine the convergence parameters are included in the provided Zenodo archive (Ref. 15).

| Simulation | $k_{\max}$ | $k_{\text{Mats}}$ | $dt$ (fs) | $\delta_A$ | $\delta_S$ | $u_t$ (fs) | $N_{\text{traj}}$ |
|---|---|---|---|---|---|---|---|
| Fig. 1a | 15 | 0/0 | 4.0 | * | * | 4.0 | 1000 |
| Figs. 1b and S1c | 15 | 0/0 | 4.0 | 0.001 | 0.001 | 4.0 | 1000 |
| Fig. 3 - No Peierls vibrations | 3 | 5/4 | 0.4 | 0 | 0 | - | 1000 |
| Fig. 3 - singlet-TT Peierls vibrations | 3 | 5/4,0/0 | 0.4 | 0 | 0 | - | 1000 |
| Figs. 3-4, 5 (dimers) - CT-TT Peierls vibrations | 3 | 10/8,0/0 | 0.2 | 0 | 0 | - | 1000 |
| Fig. 5c (trimer-hexamer) | 3 | 10/8,0/0 | 0.2 | 0.01 | 0 | 2.0 | 1000 |
| Fig. 5c (decamer) | 3 | 10/8,0/0 | 0.2 | 0.01 | 0 | 4.0 | 3000 |
| Fig. 5d - singlet MSD | 3 | 5/4 | 0.4 | 0.001 | 0.001 | 4.0 | 1917 |
| Fig. 5d-e - triplet MSD, Peierls vibrations | 3 | 10/8,0/0 | 0.2 | 0.01 | 0.005 | 4.0 | 5745 |
| Fig. 5e - triplet MSD, no Peierls vibrations | 3 | 5/4 | 0.4 | 0.001 | 0.001 | 4.0 | 5718 |
| Fig. 5f | 3 | 10/8,0/0 | 0.2 | 0.01 | 0.005 | 2.0 | 100 |
| Fig. S1a | 15 | 0/0 | 4.0 | 0.0005 | 0.001 | 8.0 | 1000 |
| Fig. S1b | 15 | 0/0 | 4.0 | 0.0005 | 0.001 | 8.0 | 1000 |

TABLE S3. The convergence parameters of all simulations. Note that in $k_{\text{Mats}}$, the form $a/b$,$c/d$ indicates the presence of two separately-parametrized types of bath, with $a$ total Matsubara modes for each Holstein bath, with $b$ of those modes Markovian-filtered, and $c$ total Matsubara modes for each Peierls bath, with $d$ of those modes Markovian-filtered. A value of * indicates that the parameter took on multiple values, specified in the figure. A value of - indicates non-applicability.

[1] Varvelo, L.; Lynd, J. K.; Bennett, D. I. G. Formally exact Simulations of Mesoscale Exciton Dynamics in Molecular Materials. *Chem. Sci.* **2021**, *12*, 9704–9711.
[2] Suess, D.; Eisfeld, A.; Strunz, W. T. Hierarchy of Stochastic Pure States for Open Quantum System Dynamics. *Phys. Rev. Lett.* **2014**, *113*, 150403.
[3] Diósi, L.; Strunz, W. T. The Non-Markovian Stochastic Schrödinger Equation for Open Systems. *Phys. Lett. A* **1997**, *235*, 569–573.
[4] Wiseman, H. M.; Gambetta, J. M. Pure-state quantum trajectories for general non-Markovian systems do not exist. *Phys. Rev. Lett.* **2008**, *101*, 140401.
[5] Citty, B.; Lynd, J. K.; Gera, T.; Varvelo, L.; Raccah, D. I. G. B. MesoHOPS: Size-Invariant Scaling Calculations of Multi-Excitation Open Quantum Systems. *J. Chem. Phys.* **2024**, *160*, 144118.
[6] A non-normalized nonlinear equation of motion may be obtained by setting $\Gamma_t$ and the associated portion of $\hat{T}$ (if applicable) to 0: in such a case, the norm of the physical wave function $\langle \psi_t^{(\vec{0})} | \psi_t^{(\vec{0})} \rangle$ is not guaranteed to go to 1. Instead, the error bounds $\delta_A$ and $\delta_S$ are replaced with $\Delta_A = \langle \psi_t^{(\vec{0})} | \psi_t^{(\vec{0})} \rangle \, \delta_A$ and $\Delta_S = \langle \psi_t^{(\vec{0})} | \psi_t^{(\vec{0})} \rangle \, \delta_S$, producing identical results.
[7] Note that in the case of an explicitly time-dependent system Hamiltonian $\hat{H}_S(t) = \hat{H}_S + \hat{W}_t$, the time-dependent portion $\hat{W}_t$ may be included as a portion of $\hat{Z}_t$ without altering the results of the derivation below.
[8] Berkelbach, T. C.; Hybertsen, M. S.; Reichman, D. R. Microscopic Theory of Singlet Exciton Fission. III. Crystalline Pentacene. *J. Chem. Phys.* **2014**, *141*, 074705.
[9] Berkelbach, T. C.; Hybertsen, M. S.; Reichman, D. R. Microscopic Theory of Singlet Exciton Fission. I. General Formulation. *J. Chem. Phys.* **2013**, *138*, 114102.
[10] Renaud, N.; Grozema, F. C. Intermolecular Vibrational Modes Speed Up Singlet Fission in Perylenediimide Crystals. *J. Phys. Chem. Lett.* **2015**, *6*, 360–365.
[11] Castellanos, M. A.; Huo, P. Enhancing Singlet Fission Dynamics by Suppressing Destructive Interference between Charge-Transfer Pathways. *J. Phys. Chem. Lett.* **2017**, *8*, 2480–2488.
[12] Volek, T. S.; Verkamp, M. A.; Ruiz, G. N.; Staat, A. J.; Li, B. C.; Rose, M. J.; Eaves, J. D.; Roberts, S. T. Slowed Singlet Exciton Fission Enhances Triplet Exciton Transport in Select Perylenediimide Crystals. *J. Am. Chem. Soc.* **2024**, *146*, 29575–29587.
[13] Berkelbach, T. C.; Hybertsen, M. S.; Reichman, D. R. Microscopic Theory of Singlet Exciton Fission. II. Application to Pentacene Dimers and the Role of Superexchange. *J. Chem. Phys.* **2013**, *138*, 114103.
[14] Varvelo, L.; Lynd, J. K.; Citty, B.; Kühn, O.; Raccah, D. I. G. B. Formally Exact Simulations of Mesoscale Exciton Diffusion in a Light-Harvesting 2 Antenna Nanoarray. *J. Chem. Phys. Lett.* **2023**, *14*, 3077–3083.
[15] Lynd, J. K.; Raccah, D. I. G. B. Figure, Input, and Analysis Scripts for "Characterizing the Role of Peierls Vibrations in Singlet Fission with the Adaptive Hierarchy of Pure States". 2025; `https://doi.org/10.5281/zenodo.15337336`.
